# Supplementary material for: Enzyme economy and metabolic control
Source: arXiv:1404.5252 source file (2022-10-04)
Supplement: Supplementary file 1 [file sec_supplement_cba_kinetic.tex]

\co{WO?

  \includegraphics[width=12cm]{../additional_material/ps-files/backpropagation1.eps}\\
  \includegraphics[width=12cm]{../additional_material/ps-files/backpropagation2.eps}\\

}

\co{

  \begin{figure*}[t!]
  \begin{center}
    \includegraphics[width=14cm]{\psfileslabourvalues/costbenefitcurves2.eps}
  \end{center}
  \caption{\co{REF IN TEXT (gibt schon ref in main article)}
    Cost-benefit and {\myvalue}-{\price} balances for enzymes.  (a)
    Cost-benefit balance. In enzyme-optimal states, the slopes of
    {\metabolicobjective} $g$ and {{\investment}} $h$ as functions of $\ln u$,
    called {{\enzymebenefit}} and {{\enzymecost}}, must be
    balanced. Since enzyme costs are positive, enzymes must have
    positive benefits, i.e.~a positive control over the metabolic
    {\metabolicobjective}.  (b) The slopes of {\metabolicobjective} and {{\investment}}
    (as functions of $u$), called enzyme {\myvalue} and {\price}, must
    also be balanced. The two terms correspond to the two paths in
    Figure \ref{fig:costbenefitcurves1} (b)).  (c) If an enzyme
    {\myvalue} is always below the {{\enzymeprice}}, the enzyme must be
    inactive in optimal states.  (d) This holds, in particular, if the
    enzyme {\myvalue} is negative.}
    \label{fig:costbenefitcurves2}
\end{figure*}

}

\coout{sagen, dass $\Cmat^{\rm g} = - {\hctot}\trans\,\Ccmat$?}

\section{Perturbed metabolic states: description by control coefficients}

\co{this has newly arrived from CBA local; check the entire section!}

\co{anfangssatz: pertrubations of metabolic steady states described by perturbation parameters and control coefficients with respect to these parameters. Here overview of all relevant types of control coefficients and their usage to handle standard metablic models in  MVT.}

\co{refer back to basic model equations (in CBA kin SI? WO?)}

\myparagraph{Systems without moiety conservation} For simplicity, let us
first consider systems without conserved moieties.  In addition to its
dependence on $\esymbolv$ and $\xv$, the metabolic state also depends on
perturbation variables $\virtgamma_{i}$, $\virtnu_{l}$,
$\virtphi_{i}$: $\virtgamma_{i}$ is added to the concentration $c_{i}$
in rate laws or in the benefit function. \co{note that psi and phi
  only apply to independent metabolit concentrations!} $\virtnu_{l}$
is added to $v_{l}$ in mass balances or in the benefit function, and
$\virtphi_{i}$ adds directly to the mass balance of metabolite
$i$. Hence, we replace:
\begin{eqnarray}
  \vv \rightarrow  \vv = \hat \vv + \virtnuv, \qquad
 \cv^{\rm ind} \rightarrow  \cv^{\rm ind}
 = \hat \cv^{\rm ind} + \virtgammav, \qquad \dot \cv \rightarrow \hat{\dot{\cv}}
 = \dot \cv + \Lmat \,\virtphiindv_{\rm ind}
\end{eqnarray}
instead of the stationarity condition
\begin{eqnarray}
  \label{eq:ModelReal}
0 = \dot \cv = \Nint\, \vv = \Nint\, \rv(\cv)
\end{eqnarray}
we now obtain 
\begin{eqnarray}
  \label{eq:ModelVirtual}
0= \dot \cv = \Nint [\rv(\hat \cv + \virtgammav) + \virtnuv] + \Lmat \,{\virtphiv}_{\rm ind}
\end{eqnarray}

\myparagraph{Metabolic control coefficients} \co{note ``sensitivities:
  direct (elasticities) and indirect (control coefficients)} By taking
the derivatives with respect to $\virtgamma_{i}$, $\virtnu_{l}$,
$\virtphi_{i}$, we obtain the derivatives for metabolic state
variables
$c_{i} = \csteady_{i}(\esymbolv,\xv,\virtgammav,\virtphiindv,\virtnuv)$ and
$v_{l} = \vsteady_{l}(\esymbolv,\xv,\virtgammav,\virtphiindv,\virtnuv)$:
\co{first definintions as derivatives!}

They read

\parbox{5cm}{
\begin{eqnarray}
C^{\cvsteady}_{\virtgammav}   & = & 0  \nonumber\\
C^{\vvsteady}_{\virtgammav}   & = & 0 \nonumber
\end{eqnarray}
}
\parbox{5cm}{
\begin{eqnarray}
C^{\cvsteady}_{\virtphiindv}  & = & - (\Nint\,\Eunc)\inv \,\Lmat \nonumber\\
C^{\vvsteady}_{\virtphiindv}  & = & \Eunc\, C^{\cvsteady}_{\virtphiindv} \nonumber
\end{eqnarray}
}
\parbox{5cm}{
\begin{eqnarray}
C^{\cvsteady}_{\virtnuv}     & = &  - (\Nint\,\Eunc)\inv \,\Nint \nonumber\\
C^{\vvsteady}_{\virtnuv}     & = & \Imat + \Eunc\,C^{\cvsteady}_{\virtnuv}.
\end{eqnarray}
}
\co{shift equation number to the right?}

\co{FN. similar definition for other state variables $p_{m}$ with corresponding virtual 
variation parameters $\psi_{m}$}

\co{WO? Control matrices: (definition in CBA I; move graphics there?)

\parbox{8cm}{\includegraphics[width=5.5cm]{/home/wolfram/projekte/cba/zeichnungen/A58.jpg}}
\parbox{8cm}{
  \begin{eqnarray}
    C^{c}_{c} &=& -(N E)\inv\nonumber \\
    C^{c}_{v} &=& C^{c}_{c} N\nonumber \\
    C^{v}_{v} &=& I + E \,C^{c}_{c} N\nonumber \\
    C^{v}_{c} &=& E \,C^{c}_{c} N
  \end{eqnarray}  
}
}

\myparagraph{Systems with moiety conservation} In a model with
conserved moieties (i.e.~a model in which $\Nint$ does not have full
row rank), we split the stoichiometric matrix into
$\Nint = \Lmat\,\NR$ and there is a left-kernel matrix $\Gmat$
satisfying $\Gmat\,\Nint=0$ and accordingly $\Gmat\,\Lmat=0$.  Each
column of $\Lmat$ refers to an independent internal metabolite and
\todo{describes metabolite changes that can be attributed to changes
  of this metabolite}. Each row of $\Gmat$ describes a conserved
moiety. For instance, if there is a conserved moiety ATP + ADP =
const, and ATP is chosen as an independent metabolite, ADP will be
dependent and there can be a column $(1,-1,0,...)\trans$ in $\Lmat$
and a row $(1,1,0, ...)$ in $\Gmat$.  The matrix $(\Lmat|\Gmat\trans)$
is quadratic and invertible. The internal concentrations can be
written as
$\cv(t) = \Lmat\,\cv^{\rm ind}(t) + \Gmat\trans\,\cv^{\rm cm}$, where
the concentrations of the conserved moieties can be determined from
the initial conditions by
$\cv^{\rm cm} = \Gmat^{+} [ \cv(0) - \Lmat\,\cv^{\rm ind}(0)]$.

In system with moiety conservation, the stationarity condition with virtual 
perturbation variables reads 
\begin{eqnarray}
  \label{eq:ModelVirtual2}
  0 = \NR\, [\rv(\hat \cv + \virtgammav) + \virtnuv] + \virtphiindv,
\end{eqnarray}
and since a virtual change $\virtgammav$ will change the conserved
moieties by exactly $\Gmat\,\virtgammav$, we obtain the additional
condition
\begin{eqnarray}
  \label{eq:ModelVirtual3}
 \frac{\partial}{\partial \virtgammav} \Gmat\,\hat \cv = 0 
\end{eqnarray}
Furthermore, we consider state variables given by algebraic equations
$\pv = \pv(\cv)$, which can also appear in the rate laws (with
elasticities $\Emat_{\pv}$) we can perturb by virtual variation
variables $\virtpsiv$.  Some other possibilities in models are not
explicitly considered here because they are already, effectively, covered by our
approach: (i) state variables $\pv$ that depend on $\cv$ and $\vv$ can
effectively be written as dependent on $\cv$ only. (ii) State
variables that are not given by algebraic, but differential equations
can be effectively be written as metabolite concentrations (with a
virtual ``producing reaction'' representing the differential equation.
With these conditions, we obtain \co{C ueberall dick!!}
\begin{eqnarray}
C^{\cvsteady}_{\virtgammav } & = & - {\NR\,\Eunc \choose \Gmat}\inv {\NR\,\Eunc \choose 0} + \Imat
= {\NR\,\Eunc \choose \Gmat}\inv {0 \choose \Gmat}
\end{eqnarray}
and thus

\parbox{8cm}{
\begin{eqnarray}
C^{\cvsteady}_{\virtgammav } & = &  {\NR\,\Eunc \choose \Gmat}\inv {0 \choose \Gmat} \nonumber \\[1mm]
C^{\cvsteady}_{\virtphiindv} & = &  - \Lmat\, (\NR\,\Eunc\,\Lmat)\inv \nonumber \\[1mm]
C^{\cvsteady}_{\virtnuv    } & = &  - \Lmat\,(\NR\,\Eunc\,\Lmat)\inv \NR\nonumber \\[1mm]
C^{\cvsteady}_{\virtpsiv   } & = & - \Lmat\,(\NR\,\Eunc\,\Lmat)\inv \NR\,\Emat_{\pv} \nonumber
\end{eqnarray}
}
\parbox{4cm}{
\begin{eqnarray}
C^{\vvsteady}_{\virtgammav } & = & \Eunc \, C^{\cvsteady}_{\virtgammav }\nonumber \\[1mm]
C^{\vvsteady}_{\virtphiindv} & = &  \Eunc\, C^{\cvsteady}_{\virtphiindv}\nonumber \\[1mm]
C^{\vvsteady}_{\virtnuv    } & = & \Eunc\,C^{\cvsteady}_{\virtnuv    } + \Imat\nonumber \\[1mm]
C^{\vvsteady}_{\virtpsiv   } & = & \Emat_{\pv} + \Eunc\,C^{\cvsteady}_{\virtpsiv    } \nonumber
\end{eqnarray}
}
\parbox{5cm}{
\begin{eqnarray}
C^{\Pv}_{\virtgammav } & = & \Emat^{\Pv}_{\cv} \, C^{\cvsteady}_{\virtgammav} \nonumber \\[1mm]
C^{\Pv}_{\virtphiindv} & = &  \Emat^{\Pv}_{\cv} \, C^{\cvsteady}_{\virtphiindv} \nonumber \\[1mm]
C^{\Pv}_{\virtnuv    } & = & \Emat^{\Pv}_{\cv} \, C^{\cvsteady}_{\virtnuv} \nonumber \\[1mm]
C^{\Pv}_{\virtpsiv   } & = & \Emat^{\Pv}_{\cv} \, C^{\cvsteady}_{\virtpsiv} +\Imat\nonumber
\end{eqnarray}
}

The derivatives with respect to $\virtnuv$ are just the usual control
coefficients, and the derivatives with respect to $\virtpsiv$ are just
the usual parameter response coefficients. For convenience, we also
define the matrices
\begin{eqnarray}
C^{\rm S}_{\virtphiv} &=& C^{\rm S}_{\virtphiindv}\,\Imat\trans_{\rm R} \nonumber \\
C^{\rm J}_{\virtphiv} &=& C^{\rm J}_{\virtphiindv}\,\Imat\trans_{\rm R}
\end{eqnarray}
where $\Imat$ is obtained from a unit matrix (corresponding to the internal metabolites) by selecting the rows corresponding to independent metabolites, such that $\NR = \Imat_{\rm R}\,\Nint$. These matrices are related to the 
usual control matrices by 
\begin{eqnarray}
C^{\rm S} &=& C^{\rm S}_{\virtphiv}\,\Nint  \nonumber \\
C^{\rm J} &=& C^{\rm J}_{\virtphiv}\,\Nint
\end{eqnarray}

\myparagraph{Effect of virtual variations on general state variables}
Consider a state variable $a$ given as a function
$\fluxcost(\vvsteady(\esymbolv,\xv,..),\cvsteady(\esymbolv,\xv,..),\Pv(\esymbolv,\xv,..))$ of the steady-state
concentrations and fluxes. Its derivatives with respect to virtual
variation variables read
\begin{eqnarray}
C^{\rm a}_{\virtgammav } & = & 
{\av^{\rm c}}\trans\, C^{\cvsteady}_{\virtgammav } + 
{\av^{\rm v}}\trans\, C^{\vvsteady}_{\virtgammav }+ 
{\av^{\rm p}}\trans\, C^{\Pv}_{\virtgammav }
= [{\av^{\rm c}}\trans + {\av^{\rm v}}\trans\,\Eunc  + {\av^{\rm p}}\trans\,\Emat^{\Pv}_{\cv}]\, C^{\cvsteady}_{\virtgammav }  
\nonumber \\
C^{\rm a}_{\virtphiindv} & = & 
{\av^{\rm c}}\trans\, C^{\cvsteady}_{\virtphiindv } + 
{\av^{\rm v}}\trans\, C^{\vvsteady}_{\virtphiindv }+ 
{\av^{\rm p}}\trans\, C^{\Pv}_{\virtphiindv }
 = [{\av^{\rm c}}\trans + {\av^{\rm v}}\trans\,\Eunc + {\av^{\rm p}}\trans\,\Emat^{\Pv}_{\cv}]\, C^{\cvsteady}_{\virtphiindv }  
 \nonumber \\
C^{\rm a}_{\virtnuv    } & = &
{\av^{\rm c}}\trans\, C^{\cvsteady}_{\virtnuv } + 
{\av^{\rm v}}\trans\, C^{\vvsteady}_{\virtnuv }+ 
{\av^{\rm p}}\trans\, C^{\Pv}_{\virtnuv }
 = {\av^{\rm v}}\trans + [{\av^{\rm c}}\trans + {\av^{\rm v}}\trans\,\Eunc + {\av^{\rm p}}\trans\,\Emat^{\Pv}_{\cv}]\, C^{\cvsteady}_{\virtnuv }  
 \nonumber \\
C^{\rm a}_{\virtpsiv    } & = &
{\av^{\rm c}}\trans\, C^{\cvsteady}_{\virtpsiv } + 
{\av^{\rm v}}\trans\, C^{\vvsteady}_{\virtpsiv } + 
{\av^{\rm p}}\trans\, C^{\Pv}_{\virtpsiv }
 = {\av^{\rm p}}\trans + [{\av^{\rm c}}\trans + {\av^{\rm v}}\trans\,\Eunc + {\av^{\rm p}}\trans\,\Emat^{\Pv}_{\cv}]\, C^{\cvsteady}_{\virtpsiv }  
\end{eqnarray}
The differential can be written as
\begin{eqnarray}
 \delta a = C^{\rm a} \, {\virtnuv}\, \delta \virtnuv + 
C^{\rm a} \, {\virtphiv}\, \delta \virtphiv + 
C^{\rm a} \, {\virtgammav}\, \delta \virtgammav + 
C^{\rm a} \, {\virtpsiv}\, \delta \virtpsiv.
\end{eqnarray}

\co{WO? EXTRA-ABSCHNITT! TEXT zu duality von CBA field SI hierher!!

  To study compound-reaction duality, we can start from the dual equations
\begin{eqnarray}
\delta \dot{\vv} &=& \Eunc\,\delta \dot{\cv} + \Eune\,\dot{\esymbolv}  \nonumber\\
\delta \dot{\cv} &=& \Nint\,\delta \vv.
\end{eqnarray}

}

\subsection{The fitness  function and its direct derivatives}

\myparagraph{\ \\Basic concepts} Our economic variables (e.g.~values and
economic potentials) are defined as derivatives of the fitness
function. When computing with them, or to establish relations between
them, we need to consider that our benefit-cost calculation is built
around dynamic models of metabolism, and therefore we need to
distinguish between basic variables like our control variables
$\esymbol_{l}$, which can be directly controlled, and state variables, whose
values are obtained by solving the dynamic system, for instance, for a
steady state depending on the basic variables.  We can write
relationships in terms of derivatives. In general, we consider a
benefit function
\begin{eqnarray}
  f(\esymbolv,\xv,\virtphiind) = z(\sv(\esymbolv,\xv,\Lmat \,\virtphiind))) - h(\esymbolv),
\end{eqnarray}
where $h$ is convex and rises monotonically in each variable $\esymbol_{l}$
(or in its absolute value, if $\esymbol_{l}$ is complex).  In a specific
interpretation, $\esymbolv$ is a vector of static enzyme levels, $\xv$ is a
vector of external metabolite concentrations, $\virtphi$ is a vector of static
virtual supply fluxes, $\sv = {\cvsteady \choose \vvsteady}$ is the vector of
steady-state internal concentrations and fluxes.  In a more relatively
general interpretation, $\esymbolv$ can contain any control variables, $\xv$
contains any uncontrollable external variables, $\sv$ is a vector of
metabolic state variables, and $z$ and $h$ are functions scoring the
variables.

\myparagraph{Economic model with separate cost function} \co{include other
  state variables $\pv = \Pv(\esymbolv,\xv)$ (algebraic (depending on c and
  p) or differential (with time derivative depending on c and p); can
  appear in reaction rates, balance equations, and benefit function)} We
first introduce the economic state variables for models with a
separate cost function.  Assume a fitness function
\begin{eqnarray}  
 \ffit(\esymbolv,\xv) = \gplus(\esymbolv,\xv) - \hminus(\esymbolv) = \bbenefit(\sv(\esymbolv,\xv)) - \hminus(\esymbolv)
\end{eqnarray}
with external variables $\xv$, control variables $\esymbolv$, metabolic state $\sv$ (comprising concentrations $\cv = \cvsteady(\esymbolv,\xv)$ and fluxes $\vv = \vvsteady(\esymbolv, \xv)$).
We define some economic variables (in column vectors) by the following  derivatives:
\co{def bv = dq/dv; gc = -dq/dc} \co{fix all the ``b'' variables below: gplus! auch fix bc : -gc}

\begin{eqnarray}
\label{eq:SomeDerivatives}
  \mbox{Enzyme economic tension}\qquad \fu &=& \partial \ffit / \partial {\esymbolv} \nonumber \\
   \mbox{Enzyme value}\qquad   \gu    &=& \partial \gplus / \partial {\esymbolv}\, \nonumber \\
   \mbox{External parameter value}\quad   \gx    &=& \partial \gplus / \partial {\xv}\, \nonumber \\
   \mbox{Enzyme loss}\qquad    \hu    &=& \partial \hminus/ \partial {\esymbolv}\nonumber  \\
   \mbox{Concentration demand}\qquad    {\bf \bbenefit}^{\rm c}    &=& \partial \bbenefit / \partial {\cv}\nonumber  \\
   \mbox{Flux demand}\qquad    {\bf \bbenefit}^{\rm v}    &=& \partial \bbenefit / \partial {\vv}\nonumber  \\
   \mbox{Concentration/enzyme response}\qquad    R^{\rm S}_{\rm u} &=& \partial \cvsteady / \partial {\esymbolv} \nonumber \\
   \mbox{Flux/enzyme response}\qquad    R^{\rm J}_{\rm u} &=& \partial \vvsteady / \partial {\esymbolv}
\end{eqnarray}
Other derivatives can be  defined accordingly. We
obtain the formulae $\fu = \gu - \hu$ and $\gu = {{\bf \bbenefit}^{\rm
    \sv}}\trans\,R^{\rm \sv}_{\esymbolv}$. To define economic variables, we
also consider derivatives with respect to virtual variations:
\begin{eqnarray}
   \mbox{Production value}\quad    \gphi &=& \delta \gplus / \delta \virtphiindv \Imat_{\rm R}\nonumber \\
   \mbox{Flux value}\qquad         \gvtot &=& \delta \gplus / \delta \virtnuv \nonumber \\
   \mbox{Concentration value}\qquad \gc   &=& \delta \gplus / \delta \virtgammav\nonumber \\
   \mbox{Other variable value}\qquad \gp   &=& \delta \gplus / \delta \virtpsiv
\end{eqnarray}

\textbf{Comprehensive economic model} We can also consider fitness
functions that do not contain a separate {{\investment}} term, but in which benefit
and {{\investment}} are combined in a single function:
\begin{eqnarray}  
 \ffit(\esymbolv,\xv) = \bbenefit(\sv(\esymbolv,\xv),\esymbolv, \xv)
\end{eqnarray}
In this case, the enzyme gain and loss from
Eq.~(\ref{eq:SomeDerivatives}) need to be redefined: 
\begin{eqnarray}
   \mbox{Enzyme value}\qquad   \gu    &=& \frac{\partial \bbenefit}{\partial \sv}\,\frac{\partial \,\sv}{\partial{\esymbolv}} \nonumber \\
   \mbox{Enzyme loss}\qquad    \hu   &=& -\partial {\esymbolv} /  \partial \bbenefit.
\end{eqnarray}
Similar other derivatives are defined accordingly.

\subsection{Economic variables}

With the virtual variations of concentrations, production rates,
fluxes, and other state variable, we can define economic values for
all these quantities:
\begin{itemize}[leftmargin=5mm]
\item \textbf{Production value} The production gain of an independent
  internal metabolite is given by the derivative $\partial
  \gplus/\partial \virtphiind_{i}$ of the metabolic benefit with respect
  to the corresponding virtual supply flux. Setting the production gains of all 
other metabolites to 0, we obtain the value vector
 \begin{eqnarray}
{\bf \gplus^{\rm \virtphiind}}\trans = {\wint}\trans = \frac{\partial  \gplus}{\partial \virtphiindv} \,\Imat_{\rm R}
 \end{eqnarray}
which we also call internal economic potential vector.
\item \textbf{Flux value} Likewise, we define the flux gain of  reaction by the 
 derivative $\partial
  \gplus/\partial \virtnu_{l}$ of the metabolic benefit with respect
  to the  virtual flux. We can write the (transposed) flux gain vector as 
 \begin{eqnarray}
{\bf \gplus^{\rm v}}\trans =   \gvtot\trans = \frac{\partial  \gplus}{\partial \virtnuv} 
= \bvtot\trans\,C^{\rm J}_{\virtnu} + {\bc}\trans\,C^{\rm S}_{\virtnu}
= \underbrace{{\bvtot}\trans}_{{(\gvdir)}\trans}  
+ \underbrace{[{\bvtot}\trans\,\Eunc + {\bc}\trans]\,C^{\rm S}_{\virtnu}}_{{\gvind}\trans},
 \end{eqnarray}
thereby splitting it into  direct and indirect flux gains. 
\item \textbf{Concentration value} The concentration gain of an internal metabolite 
is obtained from the derivative $\partial
  \gplus/\partial \virtgamma_{i}$  with respect
  to the virtual concentration variations. The vector reads
  \begin{eqnarray}
{\bf \gplus^{\rm c}}\trans =      \frac{\partial  \gplus}{\partial \virtgammav} = 
\bvtot\trans\,C^{\rm J}_{\virtgamma} + \bc\trans\,C^{\rm S}_{\virtgamma} 
= \bc\trans + 
 \underbrace{[\bvtot\trans\,\Eunc  + \bc\trans] \,C^{\rm S}_{\virtgamma}}_{{\loadint}\trans}
  \end{eqnarray}
thereby splitting it into direct concentration gain (i.e.~concentration demand)
and indirect concentration  value (i.e.~the load). Without moiety conservation,  
$\frac{\partial  \gplus}{\partial \virtgammav} $ vanishes and $\loadint = -\bc $
\item \textbf{Value of general  state variables} For algebraic state
  variables $p_{r}$, the value is defined by the derivative $\partial
  \gplus/\partial \virtpsi_{r}$ with respect to the virtual
  perturbation. This yields
  \begin{eqnarray}
{\bf \gplus^{\rm p}}\trans =    \frac{\partial  \gplus}{\partial \virtpsiv} = 
\bvtot\trans\,C^{\rm J}_{\virtpsi} + \bc\trans\,C^{\rm S}_{\virtpsi} 
= \bc\trans + 
 \underbrace{[\bvtot\trans\,\Eunc  + \bc\trans] \,C^{\rm S}_{\virtpsi}}_{{\loadint}\trans}
  \end{eqnarray}
thereby splitting it into  direct and indirect flux gains. 
\end{itemize}
\co{fix the last one and include demands for p also in other formulae.}

\section{Economic variables, rules, and balance equations}

\co{anfangssatz, sagen dass jetzt alles nochmal verbal erklaert wird,
  und mit mehr details} \co{note that full definitions of all economic
  variables (through virtual variations) are given in the supplement
  of cba local; there is also another discussion of the control
  matrices.  are all relations between the control matrices fully
  explained? is there anything new i could to conclude from these
  relations?}

Metabolic systems in optimal states can be described by economic
variables and their balance equations. To obtain such equations, we
need to understand how local perturbations (e.g.~variations of enzyme
levels) influence steady states. Economic variables (such as economic
potentials $\wint$, {\fluxvalue}s $\gvtot$, concentration {\myvalue}s
$\gc$) can be written in terms of metabolic control coefficients.
Using the framework of Metabolic Control Theory, we can define the
economic potentials as metabolic control coefficients, with the
{\metabolicobjective} as the output variable.  An alternative definition,
described in \cite{lieb:18lagrange}, is based on Lagrange multipliers:
we solve the same optimality problem, but treat rate laws and
stationarity as explicit constraints. The economic potentials and flux
{\myvalue}s can then be defined as the Lagrange multipliers associated
with these constraints (proof in section
\ref{sec:ProofsPotentialsAreIdentical}).

\begin{figure*}[t!]
  \begin{center}
\begin{tabular}{ll}
(a) Tracing the fitness effects of an enzyme & (b) Economic state variables \\
    \includegraphics[width=8cm]{\psfileskinetic/backpropagation1b.eps} & 
    \includegraphics[width=7.5cm]{\psfileskinetic/costbenefitcurves3.eps}
\end{tabular}
  \end{center} 
  \caption{\co{WO? REF IN TEXT!}  \co{ODER: a ist ergaenzte version von abb 1 a!
      a schoen in den main text einbinden. sagen, dass wir nochmal das
      scheme aus abb 1 anschauen und die genauen kausalen wirkungne
      beschreiben; mit hilfe von kontrollkoeffizienten!}  Economic
    variables associated with enzyme levels. (a) Enzyme {\myvalue}s
    describe the fitness effects of enzymes, as mediated by the
    metabolic network.  The {\myvalue} of an enzyme tells us how
    strongly a virtual variation of the enzyme level would affect the
    {\metabolicobjective} function by changing the metabolic state.  To trace such
    indirect effects, we apply the chain rule and split the total
    derivative into a series of direct derivatives (symbolically
    written as ratios of differentials
    $\frac{\delta \gplus}{\delta u} = [\frac{\delta \gplus}{\delta
      \vv} \, \frac{\delta \vv}{\delta r} + \frac{\delta
      \gplus}{\delta \cintv} \, \frac{\delta \cintv}{\delta r}]
    \frac{\delta r}{\delta u}$).  The derivatives
    $\frac{\delta \vv}{\delta r}$ and $\frac{\delta \cintv}{\delta r}$
    of steady-state variations are metabolic control coefficients.
    Metabolic value theory extends the definition of {\myvalue}s from
    model parameters (such as enzyme levels) to all metabolites and
    reactions in the network. \co{say that this tracing can now be
      inverted!}  \coout{Show formulae in table? or ref to table in
      SI?}  (b) \co{wo werden im text die point variables usw gut
      eingefuehrt?  die abbildung dorthin tun} Economic variables. In
    metabolic value theory, the scaled derivatives between {\metabolicobjective} (or
    {{\investment}}, or fitness) and an enzyme level are called
    {{\enzymebenefit}}, enzyme cost, and economic imbalance. The usual
    derivatives are called enzyme {\myvalue}s (or {{\enzymeprice}}s,
    or enzyme stresses\co{opportunity cost? thanks to ron!}).  By
    dividing the scaled derivatives by the flux, we obtain economic
    variables called {\fluxvalue}, {\fluxburden}, and flux stress.  }
  \label{fig:costbenefitcurves1} 
\end{figure*}

\subsection{Economic potentials}
\label{sec:proofenzymebenefitmetabolitevalue}

\myparagraph{\ \\Economic variables and control matrices} Using
control matrices and the chain rule, \coout{supply fluxes must have
  the form $\Lmat\,\virtphiindv$ fix the notation} the internal
economic potentials can be written as (a row vector)
\begin{eqnarray}
\label{eq:SIdefWcint}
{\wint}\trans= \Cmat^{\rm  g}_{\virtphiindv} \Lmatplus =
 [{\bvtot}\trans \Cmat^{\rm  g}_{\virtphiindv} - \hc\trans \Cmat^{\rm  g}_{\virtphiindv}]\,\Lmatplus
= [\bvtot\trans \Cvmat_{\virtphiv} - \hc\trans \Ccmat_{\virtphiv}]\trans
\end{eqnarray}
and the flux and concentration {\myvalue}s can be written as
\begin{eqnarray}
\label{eq:defGV}
\gvtot\trans &=& \Cmat^{\rm  g} = {\bvtot}\trans \Cvmat - \hc\trans \Ccmat \nonumber \\
\gc\trans    &=& \Cmat^{\rm  g}_{\virtgamma} = {\bvtot}\trans \Cvmat_{\virtgamma} 
                               - \hc\trans \Ccmat_{\virtgamma}.
\end{eqnarray}

\myparagraph{Economic potentials and reaction rule} Based on the definition of 
economic potentials, we can now prove
the {\fluxbenefitbalance} equation. Using Eq.~(\ref{eq:SIdefWcint}),
we can compute the vector of economic potential differences
\begin{eqnarray}
\label{eq:controlandvirtual1}
\Deltar \wint 
&=&  {\Nint}\trans\, \wint 
=  [\bvtot\trans \Cvmat_{\virtphiv}\, {\Nint} 
  - \hc\trans \Ccmat_{\virtphiv}\, {\Nint}]\trans 
= [\bvtot\trans (\Cvmat - \Imat) - \hc\trans \Ccmat]\trans
= \gvtot - \bvtot
\end{eqnarray}
and obtain  the equalities
\begin{eqnarray}
\label{eq:controlandvirtual1aa}
 \gvtot &=& \Deltar \wint + \bvtot = \Deltar \wint + \Deltar \wext + \bvdir = \Deltar \wtot + \bvdir.
\end{eqnarray}
By inserting Eq.~(\ref{eq:controlbysupplyproof-1}) into
Eq.~(\ref{eq:SIdefWcint}), we obtain  explicit formulae for  the  economic 
potentials and their differences
\begin{eqnarray}
\label{eq:formulawint}
{\wint}\trans &=& -  [ \bvtot \trans \Eunint - \hc \trans] \,\Lmat\, \Mmat\inv \Lmatplus 
 =  [ \bvtot \trans \Eunint - \hc\trans] \,{\Ccmat_{\virtphi}}
= -{\hctot}\trans\,\Ccmat_{\virtphiv}\nonumber \\
\Deltar \wint &=& -{\hctot}\trans\,\Ccmat_{\virtphiv} \,\Nint=
- {\hctot}\trans\,\Ccmat.
\end{eqnarray}
with the effective concentration {\price}
$\hctot = \hc - \Eunint\trans \,\bvtot$.
  \coout{WEG? Accordingly: ${\wint}\trans =
  [\bvtot\trans \,\Cv_{\virtphiindv} - \hc\trans
    \,\Cc_{\virtphiindv}]\,\Imat_{\rm R} =
  -{\hctot}\trans\Cc_{\virtphiindv}\,\Lmatplus$} 
Thus the global economic variables can be computed from local {\gain}s and {\price}s as
 \begin{eqnarray}
 \label{eq:intvalueoptcompwind6a}
 {\wint}\trans &=& - (\bvtot\trans \Eunint - \hc\trans)\, \Lmat\,(\NR \Eunint\,\Lmat)\inv\,\Lmatplus \nonumber \\
 \Deltar {\wint}\trans &=& 
- (\bvtot\trans \Eunint - \hc\trans)\, \Lmat \,(\NR \Eunint\,\Lmat)\inv\,\NR.
 \end{eqnarray}
These formulae also apply to  models with non-enzymatic reactions and dilution.  
\coout{ We can now consider two special cases.  If the metabolic objective
 $\bbenefit(\vv)$ scores only fluxes, we obtain
 \begin{eqnarray}
 \label{eq:intvalueoptcompwind2}
 {\wint}\trans &=& \bvtot\trans \Cvmat_{\virtphi} = - \bvtot\trans \Eunint \Lmat\, (\NR \Eunint \Lmat)\inv\, \Lmatplus \nonumber \\
 \label{eq:intvalueoptcompwind3}
 \Deltar {\wtot}\trans &=& 
 {\wint}\trans \Nint 
 = - \bvtot\trans \Eunint \Lmat\, (\NR \Eunint \Lmat)\inv \NR 
 = \bvtot\trans (\Cvmat-\Imat) = \bvtot\trans \Cvmat - \bvtot\trans. 
 \end{eqnarray}
and if the metabolic objective $\bbenefit(\cintv)$ scores only internal
 concentrations, 
 \begin{eqnarray}
 \label{eq:intvalueoptcompwind4}
 {\wint}\trans &=& -\hc\trans \Ccmat_{\virtphi} =  \hc\trans \Lmat\, (\NR \Eunint \Lmat)\inv\,\Lmatplus \nonumber \\
 \label{eq:intvalueoptcompwind5}
 \Deltar {\wtot}\trans &=&  \hc\trans \Lmat(\NR \Eunint\,\Lmat)\inv \NR = -\hc\trans \Ccmat.
 \end{eqnarray}}

\myparagraph{Economic potentials in models with dilution} \co{Note
  that an example (small growing cell) is currently in CBA
  Lagrange. should this example be moved here? nee lieber referenz!}
To compute feasible economic potentials $\winti$ and flux demands
$g^{\rm v}_{l}$ for a given network model with dilution, we use the
reaction rule and the metabolite rule for models with dilution (but
without moiety conservation): 
\begin{eqnarray}
\label{eq:formulaForComcentrationValues0}
  \gvtot &=& {\Nint}\trans \wint + {\Next}\trans \wext + \bvdir\nonumber \\
\hc &=&\Eunc \trans \gvtot - \lambda \, \wint.
\end{eqnarray}
Given the external economic potentials and the growth rate $\lambda$,
we can solve for the internal economic potentials.  By combining the
rules Eq.~(\ref{eq:formulaForComcentrationValues0}), we obtain
 \begin{eqnarray}
\label{eq:formulaForComcentrationValues}
 0 &=& 
 -\hc +\Eunc \trans [{\Nint}\trans \wint + {\Next}\trans \wext + \bvdir]
  - \lambda \, \wint \nonumber \\
\Rightarrow \quad \wint
  &=& - 
 ((\Nint\Eunc - \lambda\, \Imat)\trans)\inv [-\hc+\Eunc\trans\,[{\Next}\trans \,{\wext + \bvdir]]} \nonumber \\
 &=& - (\underbrace{(\Nint\Eunc - \lambda\, \Imat}_{\Mmat_\lambda})\trans)\inv 
\underbrace{[ -\hc +\Eunc\trans\, \bvtot]}_{-\hc^{\rm eff}}.
 \end{eqnarray}
 For a solution to exist the system must be dynamically stable and the
 Jacobian matrix $\Mmat_\lambda$ must be invertible.

\myparagraph{Conserved moieties and the gauging of economic
  potentials}
\label{sec:conservedmoieties}
Depending on network structure, there can be conserved
moieties in a model. For instance, if ADP and ATP are only interconverted, but never
produced or consumed individually, their total concentration [ATP]+[ADP]
remains  constant in time.  Conserved moieties are associated with
left-kernel vectors of the internal stoichiometric matrix $\Nint$.
Metabolites that share a conserved moiety have dependent
concentrations. To account for this in our models, we can choose a set of independent
metabolites (concentration vector $\cintv'$) that uniquely determine all
metabolite concentrations. The concentration changes of all
metabolites can be written as
$\md \cintv /\md t = \Lmat\, \md \cintv' /\md t$, with a link matrix $\Lmat$
satisfying $\Nint = \Lmat \, \NR$.  Each conserved moiety is associated
with a vector $\gv_{\rm cm}$ satisfying
$\gv_{\rm cm}\trans \Nint = 0$. We can write such vectors as
$\gv_{\rm cm} = \Gmat\trans\,\qv$, with a left-kernel matrix $\Gmat$
satisfying $\Gmat\,\Nint=0$. For metabolic value theory, moiety
conservation has several consequences:
\begin{enumerate}[leftmargin=5mm]
\item To define the economic potentials of internal metabolites,
  we introduce virtual supply fluxes. In models with moiety
  conservation, the virtual supply fluxes must be chosen such that
   conserved
  moieties are not affected (otherwise, they would create a non-steady
  state).  To satisfy this condition, a vector of  virtual supply fluxes must have the
  form $\virtphiv = \Lmat\,\virtphiindv$, based on virtual supply
  fluxes $\virtphiindv$ for independent metabolites.  With these
  supply fluxes, we can define the economic potentials for independent
  internal metabolites, while the dependent internal metabolites are defined to have
  vanishing economic potentials.

\item To define the  economic potentials in a kinetic model, we need to refer
  to a specific choice of independent metabolites. This means that there is some freedom in the choice of economic potentials. In the flux benefit balance, economic potentials do
  never appear separately, but only in the form of differences $\Delta
  \wtot$. As a consequence, if metabolites form a conserved moiety,
  their economic potentials can be gauged: adding a conserved moiety
  vector $\gv_{\rm cm}$ to the internal economic potential vector ($\wint
  \rightarrow \wint+\gv_{\rm cm}$) does not change the economic
  balances\footnote{If we  define a conserved moiety vector
    $\gv_{\rm cm}$ among all (internal and external) metabolites,
    it will satisfy $\gv_{\rm cm}\trans \Ntot = 0$ and 
    ${\Ntot}\trans [\wtot+\gv_{\rm cm}] = {\Ntot}\trans \wtot$. However,
    adding such a conserved moiety vector will change the external
    economic potentials and thus, the assumed production {\gain}s of
    external metabolites.}  because ${\Nint}\trans [\wint+\gv_{\rm cm}] =
  {\Nint}\trans \wint$.  If metabolites do not participate in active
  reactions, their potentials are irrelevant and can be freely gauged.
  \coout{\item A similar thing holds for the economic loads in the
    compound balance. A compound balance exists for each independent
    metabolite; however, the dependent metabolites are not completely
    irrelevant, but appear in the equation of the metabolites on which
    they depend; both are connected, again, by the link matrix. Again,
    the balance equations do not determine the loads uniquely and
    there remains a gauge freedom $(\loadint \rightarrow \loadint +
    \gv)$ for the economic loads of metabolites forming conserved
    moieties.}
\end{enumerate}
When we estimate economic potentials from measured data, we need to 
remember this gauge freedom: for example, if ATP+ADP is a conserved
moiety, observed enzyme investments will never allow us to determine
the individual economic potentials of ATP and ADP, but only their
difference.  \coout{WIRKLICH? if a {\flow} consists of several
  disconnected parts (not connected by any internal nor external
  metabolites), the potentials within each part can also be regauged.}

\subsection{Economic potentials  derived from the flux variation condition}
\label{sec:FluxVariationConditionLeadsToEconomicPotentials}

In the article, the economic potentials were defined as control
coefficients, and the economic balance equations show that the
potentials, in optimal states, are equal to ``embodied values''
related to enzyme investments. But we can also get to a notion of
economic potentials directly, by starting from a very idea of embodied
values, and based solely on the flux variation condition.  In a linear
metabolic pathway, by summing all enzyme investments upstream of a
metabolite, we obtain the ``embodied enzyme investment'' in that
metabolite, and dividing this by metabolite production rate (i.e.~the
pathway flux), we obtain the ``embodied value'' of that
metabolite. However, this definition works only for linear chains,
where investments simply accumulate from reaction to reaction. But we
can generalise the notion of ``embodied values'' to metabolites in
general networks, with branched and cyclic fluxes. To do so, we
consider the flux variation condition and \co{also refer to more
  elegant proof (and the corresponding proof for
  {\connectivitycondition} and {\compoundbenefitbalance}) in
  \ref{sec:fromSumFormulaToLocal}} \todo{\co{besserer uebergang!
    lieber sagen: cumulative value von linearer kette auf anderes
    verallgemeinern!  nochmal sagen, wo wir tstarten, naemlich bei den
    var cond!}  Let me restate this less technically and show how we
  can get to the notion of economic potentials.} Intuitively, in the
{\summationcondition} we ``probe'' the system with stationary flux
variations and compare the changes in cost and benefit. For optimality
reasons, the two changes must be equal for any possible flux variation
(because they must be equal for any enzyme variation that might have
causes the flux variation). Can we apply this principle also to
non-stationary flux variations, e.g.~a flux variation in a single
reaction? And can we apply similar optimality conditions to other
network elements, to define a notion of ``value'' for metabolites,
instead of enzymes? The cumulative {\fluxvalue}s in Figure
\ref{fig:unbranchedfluxART}, an example of such values, can be
generalised from linear pathways to metabolic networks. Using the
{\summationcondition} Eq.~(\ref{eq:fitnessbalance2x}), we can express
the cost of each enzyme by a value difference between its substrates
and products.  Given $v_l$, $\hudotl$, and $\bvtotl$, we define the
economic potential differences
\begin{eqnarray}
\label{eq:defDeltaW}
  \Deltar \wintl = \hudotl/v_l-\bvtotl.
\end{eqnarray}
As suggested by the symbol, $\Deltar \wint$ is a difference
$\Deltar \wint = \sum_i n_{il}\, \winti$ of quantities $\winti$
associated with metabolites (where only \emph{internal} metabolites
are considered in the difference). We can prove this mathematically by
showing that $\kv\trans\,\Deltar \wint=0$ for all kernel vectors $\kv$
satisfying $\Nint\,\kv=0$; this follows directly from the
{\summationcondition}.  By rearranging Eq.~(\ref{eq:defDeltaW}), we
obtain 
\begin{eqnarray}
(\Deltar \wintl + \bvtotl)\,v_l= \hudotl.
\end{eqnarray}
To rewrite this in terms of economic potentials in general (not only
internal economic potentials), we use
Eq.~(\ref{eq:splitmarginalfluxbenefit}) to split $\bvtotl$ into
$\bvtotl = \Deltar \wextl + \bvdirl$ (where only external metabolites
are considered in $\Deltar \wextl$). By setting
$\Deltar \wtotl = \Deltar \wintl + \Deltar \wextl$ (where \emph{all}
metabolites are considered in $\Deltar \wtotl$), we obtain the
economic reaction balance
\begin{eqnarray}
\label{eq:FluxBenefitBalanceFirst}
(\Deltar \wtotl + \bvdirl)\,v_l= \hudotl.
\end{eqnarray}
The term in brackets, called {\fluxvalue} $\gvtotl$, represents the
total {\myvalue} for the reaction flux $v_l$. the formula shows that
it consists of a direct {\myvalue} $\bvdirl$, which directly scores
the flux, and an indirect {\myvalue} $\Deltar \wtotl$, which scores
the global fitness effects of this flux, as mediated through direct
production and consumption of reactants. This is the economic flux
rule. \co{these are the same economic potentials as those defined by
  control coefficients} \co{note that, in the same way, the economic
  loads can be derived (stimmt das? wie?)}

\co{ REF TO THIS, WO? Direct derivation of metabolite variation condition (and local metabolite balance) from connectivity theorem:

  \subsection{Economic potentials  derived from the metabolite  variation condition}
\label{sec:MetaboliteVariationConditionLeadsToMetaboliteBalance}

  Def Flux value ${w^{tot}}\trans = b_{v}\trans + (-g_{c}\trans + b_{v}\trans\,E_{c}) \,C^{c}$

  Connectivity theorem: $C^{c}\,E_{c}\,L =-L$

  Right-multiplying (1) by $E_{c}\L$ and usin gthe theorem yields
  
  ${w^{tot}}\trans\, E_{c}\,L= b_{v}\trans\, E_{c}\,L - (-g_{c}\trans + b_{v}\trans\,E_{c}) \,L = g_{c}\trans\,L$

  Since in optimal state, $w^{tot} = a_{v}$, we obtain the metabolite variation
  condition

  $(g_{c} + E_{c}\trans a_{v}) \,L= 0$

In models without moiety conservation (where $L=I$), this yields one separate equation for each metabolite. For models with moiety conservation, we can modify the condition, to obtain separate equations.
  
We  use the fact that $(L,G\trans)$ is invertible (since $L$ and $G\trans$ have orthogonal columns, and the right number of columns).

Then we can argue that
\begin{eqnarray}
  (g_{c} + E_{c}\trans a_{v})\, \perp \boldsymbol{\ell}= 0
\end{eqnarray}
for all ${\ell} \in span(N)$, i.e.~possible columns of $L$. Since $span(G\trans)\perp span(L)$, we
obtain
\begin{eqnarray}
  (g_{c} + E_{c}\trans a_{v})\, \in span(G\trans) \nonumber \\
  (g_{c} + E_{c}\trans a_{v}) + G\trans \,w_{cm} = 0
\end{eqnarray}
for a suitable chocie of $w_{cm}$. This yields a local equation for each metabolite!

ALSO refer to this in CBA lagrange (when referring back to (not really local)
optimality condition in CBA opt)
}

\subsection{Economic loads}

\myparagraph{\ \\Metabolite rule for models with conserved moieties} If
an internal metabolite concentration  is perturbed (by adding a certain amount
of the metabolite in one moment), a system may be able return to its
original state. However,  this is not always the case: if a conserved moiety
is affected, this perturbation cannot be undone by the system
dynamics. To describe this, we can split the original perturbation
into a ``controllable'' part that is cancelled and a
``non-controllable'' part that remains and leads to a change of 
 the metabolite  concentrations 
involved in conserved moieties.  By considering a small variation of
the metabolite concentrations (in a vector $\delta \virtgammav$) and tracing
its fate, we can derive the metabolite rule. Here are two possible
derivations.

\textbf{Metabolite rule (Derivation 1):}
The direct effect on 
reaction rates,  $\delta \vv = \Eun\, \delta\virtgammav$, would 
change the fitness by $\gvtot\trans\,\Eun\,\delta \virtgammav$ where
$\gvtot=\Deltar \wtot+\bvdir$.  The local fitness balance thus reads
\begin{eqnarray}
  \delta \gplus = -\hc\trans\,\delta \virtgammav + 
\gvtot\trans\,\Eun\,\delta \virtgammav.
\end{eqnarray}
The same fitness change can also be written in terms of the concentration {\myvalue}s
\begin{eqnarray}
  \delta\gplus = \gc \cdot \delta \virtgammav.
\end{eqnarray}
By equating both formulae and dividing by 
$\delta \virtgammav$, we obtain the metabolite rule
\begin{eqnarray}
{\gc}\trans  \hc\trans = \gvtot\trans\,\Eun.
\end{eqnarray}

\textbf{Metabolite rule (Derivation 2):}
\label{sec:proofecloadcongain}
In our second, alternative derivation, we consider a virtual initial
concentration variation $\delta \virtgamma_i$ of an internal
metabolite. Its marginal effect on the {\metabolicobjective} function $\gplus$
is given by $\gci = \frac{\partial \gplus}{\partial \virtgamma_{i}}$,
which defines the concentration {\myvalue} $\gci$.  In models without
moiety conservation, the system dynamics allows the metabolites to
return to their initial steady state concentrations. In models with
moiety conservation, perturbations of conserved moieties cannot be
undone, and they may permanently change the   {\metabolicobjective}. With the
control matrices $\Cvmat_{\virtgamma}$ and $\Ccmat_{\virtgamma}$ (see section
\ref{sec:SIvirtualVariations}), the
resulting concentration {\myvalue}s can be written as
\begin{eqnarray}
  \label{eq:economicLoad2}
{\gc}\trans = \bvtot\trans\, \Cvmat_{\virtgamma} - \hc\trans \, \Ccmat_{\virtgamma}
 = [\bvtot\trans\, \Eunint - \hc\trans] \, \Ccmat_{\virtgamma}
 = -{\hctot}\trans\, \Ccmat_{\virtgamma}.
\end{eqnarray}
By applying the connectivity theorem from {\MCA}, we can see that it satisfies
${\gc}\trans\Lmat=0$ (see \ref{sec:SIvirtualVariations}).  As shown in
SI \ref{sec:loadproof}, we can further split it into a sum
\begin{eqnarray}
  \label{eq:economicLoad2}
\gci =  -\hci + \sum_l C^{\rm g}_l\, \Eunvlci.
\end{eqnarray}

\myparagraph{The economic load} The \emph{indirect} concentration
value of an internal metabolite $i$, called its economic load
$\loadi$, is given by the total concentration {\myvalue} $\gci$ minus
the direct concentration value (i.e.~the negative metabolite {\price}
$\hci$), that is $\loadi = \gci + \hci$.  The economic load appears
like an effective concentration {\price} promoted by the system,
i.e.~by the fact that the metabolite concentration has a direct effect on
neighbouring reaction rates, and via these rates an effect on the
steady state and on the {\metabolicobjective}.  The metabolite
rule (\ref{eq:economicLoad2}) tells us that the load
$\loadi = \gci + \hci$ can also be written as
$\loadi = \sum_l \gvtotl\, \Eunvlci$.  The vector of internal loads is
therefore given by 
\begin{eqnarray}
  \label{eq:economicLoad}
{\loadint}\trans = \Cmat^{\rm g}\, \Eunint = \bvtot\trans \,\Cvmat \,\Eunint - \hc\trans \,\Ccmat \,\Eunint.
\end{eqnarray}
By multiplying the load vector with the link matrix $\Lmat$ and
applying the connectivity theorem, we obtain the equality
\begin{eqnarray}
\label{eq:proofecloadcongain1}
{\loadint}\trans\,\Lmat = [\bvtot\trans\,\Cvmat -
\hc\trans\,\Ccmat] \,\Eun\,\Lmat = \hc\trans \,\Lmat.
\end{eqnarray}
In models without moiety conservation (i.e.~$\Lmat=\Imat$), this
implies that $\loadint = \hc$ and $\gc=0$.

\subsection{Economic variables in general}

\myparagraph{\ \\Economic {\fluxvalue}s can be obtained from local
  {\gain}s and {\price}s by projection} The formulae
Eqs~(\ref{eq:SIdefWcint}) and (\ref{eq:economicLoad}) for economic
variables show that the global flux and concentration {\myvalue}s can
be obtained from projections of local {\fluxgain}s and concentration
{\price}s: in models with flux objective ($\hc=0$),
Eq.~(\ref{eq:defGV}) shows that the {\fluxvalue} vector
$\gvtot = {\Cvmat}\trans\, \bvtot$ is obtained by applying the
transposed flux projector to the {\fluxgain} vector
$\bvtot$. Similarly Eq.~(\ref{eq:economicLoad2}) shows that the
concentration {\myvalue} vector is obtained as
$\gc = {\Cvmat_{\virtgamma}}\trans \,\bvtot -
{\Ccmat_{\virtgamma}}\trans \,\hc = -
{\Ccmat_{\virtgamma}}\trans\,\hctot$, i.e.~by applying the transposed
concentration projector to the effective proximal concentration
{\price} $\hctot = \hc - {\Eunint}\trans\,\bvtot$.  This holds for any
objective function.

\myparagraph{Potentials and loads can be defined for any state
  variables and functions} \co{gut in paper erwaehnt?} Also another
trick -- rewriting control coefficients as local differences -- works
not only in the case of flux values, but for any differentiable
function $f(\vv,\cintv)$ of the state variables -- including the state
variables themselves, any benefit functions, or even likelihood
functions that relate model predictions to experimental
data. Any such output
variable defines a set of economic potentials.  Given the function
$f(\cintv, \vv)$, we can write its control coefficients as
\begin{eqnarray}
 \Cmat^{\rm f}_{v} &=& ({\fv_{c}}\trans \Ccmat+{\fv_{v}}\trans \Cvmat) = \fv_{v} + ({\fv_{c}}\trans + {\fv_{v}}\trans \Eunint)\, \Ccmat \nonumber\\
&=& \fv_{v} + {\fv_{c*}}\trans\,\Ccmat_{\virtphiind}\,\NR = \fv_{v} + {\wv^{(f)}}\trans\, {\NR}
\end{eqnarray}
with $f_{v_{l}}= \partial f/\partial v_{l}$ and $f_{\cint_{i}}=
\partial f/\partial \cint_{i}$ (direct flux or concentration effects on
$f$), the proximal concentration effects $\fv_{c*}=\fv_{c}\trans +
\fv_{v}\trans \Eunint$, and  $\wv^{(f)} =
     {\Ccmat_{\virtphi}}\trans\,\fv_{c*}$ (internal potentials with
     respect to the variable $f$).  Analogous definitions can
      be given for  other economic variables, such as flux or
     concentration {\myvalue}s or economic loads.

     \co{emphasise likelihood this in paper?} \co{WO?  maybe as an
       example where the splitting of control coefficients is
       explained. // \textbf{Model fitting} In the economic balance
       equations, a global objective (e.g.~represented by flux
       {\gain}s in some distant reaction) is replaced by local proxy
       variables (e.g.~economics potentials). The same trick can also
       be used for model fitting. Imagine that we aim to fit our cell
       model to given flux, metabolite, and enzyme data \co{But what
         about enzyme cost - would it also arise from a least-squares
         fit?  is it a problem that the costs may be non-positive?}
       by maximising the negative weighted sum of squared residuals
\begin{eqnarray}
  \label{eq:fluxesclosetodata}
F(\vv,\cv,\esymbolv) =
    - \underbrace{\sum_{l} \frac{(v_{l}- v^{\rm exp}_{l})^{2}}{(\sigma^{\rm v}_{l})^{2}}}_{-\fluxcost(\vv)}
   - \underbrace{\sum_{i} \frac{(c_{i}- c^{\rm exp}_{i})^{2}}{(\sigma^{\rm c}_{i})^{2}}}_{\metcost(\cv)}
   - \underbrace{\sum_{l} \frac{(u_{l}- u^{\rm exp}_{l})^{2}}{(\sigma^{\rm u}_{l})^{2}}}_{\hminus(\esymbolv)}.
\end{eqnarray}
We can use this an a hypothetical fitess function! The only difference
is that now the ``enzyme {\price}s'' $\hul$ may not be strictly
positive; this means, for example, that the fluxes may also lead from
higher to lower economic potentials. Aside from this detail, all
economic variables can be defined (telling us how changes in the
simulated metabolic state would improve the fit), and the economic
balance equations will hold. The equations tell us about how different
model variables ``compete'' in contributing to the goodness of fit.}

\subsection{Reaction rule: writing control coefficients as differences
  along reactions}
\label{sec:SIderivationReactionRule}

To derive the reaction rule, we express the
economic variables by metabolic control coefficients:
\begin{eqnarray}
   \label{eq:enzymebalance0A}
\gu\trans\,  \diag(\enzymev/\vv)
&=& {\bvtot}\trans\, \Cvmat - \hc\trans \, \Ccmat  \nonumber \\
&=& {\bvtot}\trans\, (\Imat + \Eunc\, \Ccmat) - \hc\trans \, \Ccmat  \nonumber \\
&=& {\bvtot}\trans + ({\bvtot}\trans\,\Eunc - \hc\trans) \, \Ccmat \nonumber \\
&=& {\bvdir}\trans + \underbrace{{\bpsi}\trans}_{{\wext}\trans}\,\Next
    + \underbrace{({\bvtot}\trans\,\Eunc - \hc\trans) \, \Ccind_{\virtphi}}_{{\wint}\trans}\,\Nint  %\nonumber \\
%&=& {\bvdir}\trans + {\wint \choose \wext}\trans {\Nint \choose  \Next} \nonumber \\
= {\bvdir}\trans + \Deltar \wtot.
\end{eqnarray}
\co{die herleitung ist zu detailliert? formel ins SI, hier nur
  $\Ccmat = \Ccmat_{\virtphi}\,\Nint$ verraten} \co{ALLG: the fact
  that the indirect flux value can be written as a difference of
  production values comes from $\Ccmat = \Ccmat_{\virtphi}\,\Nint$}
\co{formel erklaeren, REF to SI} The same trick -- writing economic values
associated with reaction as a difference of economic values
associated with  metabolite production in that reaction
-- can be applied  generally, even if  $f$ is for instance a likelihood
function, scoring possible model states by comparing them to
experimentally measured state variables: \co{was kommt dabei raus?}
all control coefficients (for any differentiable function
$f(\vv,\cintv)$ of the state variables $\vv$ and $\cintv$) can be
written as local differences
\co{$\Cmat^{\rm a}_{v} = \av^{v} + \bv\trans\, {\NR}$} of ``compound
control coefficients''. \co{WORT!}  (see SI
\ref{sec:proofeconomicalternative}).  \co{kann man die metabolitregel
  mit einem aehnlichen {\MCA}-trick erklaeren?}

\subsection{Economic laws in their different forms}

\myparagraph{\ \\Different formulations of the economic balance
  equations} The economic balance equations describe how variations of
the metabolic state affect cell fitness. Variations can be described
in various ways, as differential or finite changes of state variables,
or directly in terms of fitness derivatives. Accordingly, the economic
laws can be given in different forms.  For example, the reaction
balance can be written in four different formulations, referring to
(i) enzyme {\myvalue} and enzyme {\price}, (ii) {\fluxvalue} and
{\fluxburden}, (iii) {\enzymecost} and {\enzymebenefit}, or (iv)
differential enzyme cost and differential enzyme benefit.  To derive
these formulations, we start from the enzyme {\myvalue}-{\price}
balance $\gu = \hu$. By inserting
$\gu\trans = \Cmat^{\rm g}\, \diag(\vv)\diag(\esymbolv)\inv$ and multiplying
with different variables from the right (and the symbols
$\odots$ and $\oslashs$ for componentwise vector multiplication and division)
\begin{eqnarray}
\Cmat^{\rm g}\, \diag(\vv\oslashs\esymbolv) &=& \hu\trans \nonumber \\
\Cmat^{\rm g} &=& \hu\trans \,\diag(\esymbolv\oslashs\vv)\nonumber \\
\Cmat^{\rm g}\, \diag(\vv) &=& \hu\trans \,\diag(\esymbolv) \nonumber \\
\Cmat^{\rm g}\, \diag(\delta \vv) &=& \hu\trans \,\diag(\esymbolv\oslashs\vv\odots\delta \vv) = \hu\trans \,\diag(\delta \esymbolv)
\end{eqnarray}
Similarly, starting from
${\Cmat^{\rm g}}\trans = \gvtot = \Deltar \wtot + \bvdir$, we obtain
four formulations of the reaction balance: \co{die formeln kommen
  jetzt auch in appendix; hier weg?}
\begin{eqnarray}
  \left[\Deltar \wtot + \bvdir\right] \odots \vv \oslashs \esymbolv &=&  \hu \quad\qquad\qquad\qquad\mbox{Enzyme \valueform}\nonumber \\
  \Deltar \wtot + \bvdir &=&  \hu \odots \esymbolv \oslashs \vv = \hvv \qquad\mbox{Flux \valueform}\nonumber \\
  \left[\Deltar \wtot + \bvdir\right] \odots \vv &=&  \hu \odots \esymbolv = \hudot \quad\qquad\mbox{Partial \pointbenefitform}\nonumber \\
  \left[\Deltar \wtot + \bvdir\right] \odots \delta \vv &=&  \hu  \odots \delta \esymbolv =\delta \hudot \qquad\mbox{Differential \pointbenefitform}
\end{eqnarray}
Given the reaction balance in \enzymevalueform, all other forms can
be simply obtained by multiplying with $u$, $u/v$, or $\delta
u$. \co{entsprechende formulierungen for
  other balance equations, rules, etc. // Example:
  $-\cintv \odots \hc = -\sum_l \Escint \hudot \hc = \cintv\inv \odots
  [\Escint\, \hudot] = \Eunint\,\acostv$ ???}

\section{Variants of the economic laws for more complicated models}
\label{sec:extensions}

In the article, we have made many simplifying assumptions about our kinetic
models (e.g.~each reaction must be catalysed by a specific enzyme) and
optimality problems  (e.g.~metabolite concentrations are scored by a cost, but are not
constrained by hard bounds).  We now drop some of these assumptions to make the theory
 applicable to a wider range of models or optimality problems.

\subsection{Isoenzymes and unspecific enzymes}
\label{sec:isoenzymes}
\label{sec:SIreactionBalanceNonUniqueEnzymes}

So far, we assumed that reactions are enzyme-catalysed and that
enzymes are fully specific (``unique enzyme assumption'').  In
reality, enzymes may catalyse several reactions, and reactions may be
catalysed by several enzymes. To consider this in models, we can split
each reaction into ``isoreactions'' (related to different isoenzymes)
and each enzyme into ``isoenzymes'' \co{schlechtes wort! ``enzyme
  subpools''? ueberall aendern} such that each enzyme subpool
catalyses, specifically, one single isoreaction.  Isoreactions have
identical reaction formulae and therefore identical
{\fluxvalue}s. Summing over their reaction balances (with indices $l$
for different isoenzymes), we obtain a joint reaction balance (index
$L$)
\begin{eqnarray}
 [w^{\rm v}_{L} + \Deltar w_{L}] \,v_{L} = \sum_{l \in L} \hul\,u_{l}.
\end{eqnarray}
The isoenzymes can
be replaced by a single enzyme with level $u_{L}=\sum_l u_{l}$ and
{{\enzymeprice}} $h^{u}_{L} = \frac{\sum_{l} \hul\,u_{l}}{\sum_{l}
  u_{l}}$.  

To describe unspecific or multifunctional enzymes, we need to modify  the
flux benefit balance equation. Consider an enzyme (index $l$) that
catalyses several reactions (indices $j \in J(l)$). In the reaction
balance, we sum the point benefits of all  reactions:
\begin{eqnarray}
 \label{eq.multifunctionalenzyme}
 \sum_{j \in J(l)} [\Deltar \wtotj + w^{\rm v}_{j}]\,v_{j} = \hul\, u_{l}.
\end{eqnarray}
This summation has two effects.  First, if all these reactions have
positive {{\enzymebenefit}}s, the {{\costshade}}s for all
multifunctional enzymes will be higher than for a monofunctional
enzyme.  This is plausible: if more substrates compete for the enzyme,
then more of the enzyme will be needed to catalyse all reactions
(which justifies the higher enzyme investment).  Second, there may
also be enzymes that co-catalyse deleterious side reactions.  Such
reactions would normally not occur, but if the overall enzyme benefit
remains positive, they can be active in optimal states, despite their
negative benefit, as an inevitable side effect.

%\subsection{Economic balance equations with unspecific enzymes and isoenzymes}

We have seen that we can satisfy the unique enzyme assumption by
splitting reactions and enzymes into separate ``isoreactions'' and
``isoenzymes'' with a unique mapping between them.  But this
duplication of network elements may cause problems: for example,
several copies of a reaction will have exactly the same kinetics, and
therefore the metabolite elasticity matrix will not have full column
rank.  Thus, alternatively we may keep our reactions and enzymes, with
the non-unique mapping between them. How can we derive the reaction
balance in such models? The elasticity matrix $\Eunu$ will not be
diagonal, and maybe not even quadratic. The benefit-cost condition for
enzyme levels reads
\begin{eqnarray}
\label{eq:BalanceNonUniqueCondition1}
\gvtot\trans \Eunu &=& \huv\trans.
\end{eqnarray}
Let us assume that the 
enzyme {\price} vector $\huv$ is predefined and that we search for a solution $\gvtot$.
For a solution to exist,
$\huv$ must be in the span of ${\Eunu}\trans$, and since $\huv$ can be
freely chosen, this means that $\Eunu$ must have full column
rank. \co{does this mean, if an enzyme catalyses no reaction, it must
  be switched off? or what does it mean precisely?} With the scaled
elasticity matrix $\Escu$, we can rewrite
Eq.~(\ref{eq:BalanceNonUniqueCondition1}) as
\begin{eqnarray}
\gvtot\trans \diag(\vv)\Escu &=& \huv\trans\,\diag(\esymbolv),
\end{eqnarray}
and by multiplying with the pseudoinverse
${\Escu}~^{+} = {\Escu}~\trans(\Escu\,{\Escu}~\trans)\inv$, and
redefining the {fluxburden}s\footnote{Instead of the pseudoinverse,
  we could also choose any matrix of the form
  ${\Escu}~^{+'} = {\Escu}~^{+'} + \mbox{Ker}(\Escu)\,\Amat$, with some
  arbitrary matrix $\Amat$. However, since we assumed that
  $\diag(\esymbolv)\, \huv$ is in the span of $\Escu$, it must be orthogonal
  to $\mbox{Ker}(\Escu)$ and therefore this extra term has no effect.}
as $\acostv = \huv\trans\,\diag(\esymbolv)\,{\Escu}~^{+}\, \diag(\vv)\inv$,
we obtain the well-known equality
\begin{eqnarray}
\gvtot\trans &=& \acostv.
\end{eqnarray}

\subsection{Bounds on the state variables give rise
  to shadow {\gain}s and shadow {\price}s}
\label{sec:inequality constraints}

In metabolic value theory, we assume that $u_{l} \ge 0$, i.e.~that enzyme
levels cannot be negative. Similar constraints may be imposed, for
instance, to keep metabolite concentrations in physiological ranges, to
enforce some basal rate in ATP-consuming maintenance reactions, or to limit
the total enzyme density in compartments or on cellular membranes
\cite{zhvm:11}. \co{another case?: impose dilution, by setting
  $\Nint\,\vv \ge \lambda\,\cintv$} In a general form, these
constraints can be written as linear inequalities
\begin{eqnarray}
\label{eq:hardconstraints1}
\Amat_{\rm v}\, \vv + \Amat_{\rm c}\, \cintv + \Amat_{\rm u}\, \esymbolv \ge \bv, \qquad
\end{eqnarray}
In  enzyme optimisation, active inequalities are associated with 
Lagrange multipliers. To find an optimal state,  we can maximise the Lagrangian
\begin{eqnarray}
\label{eq:hardconstraints2}
{\mathcal L}(\esymbolv) = \ffit(\esymbolv) + \betav\trans \left[\Amat_{\rm v}\, \vvsteady(\esymbolv) 
+  \Amat_{\rm c}\, \cvsteady(\esymbolv) +  \Amat_{\rm u}\, \esymbolv \right]
\end{eqnarray}
with Lagrange multipliers in vectors $\betav$.  In the solution, the
Lagrange multipliers for active lower bounds will be positive , those
for active higher bounds will be negative, and those for inactive
bounds will vanish.  The resulting cost-benefit balance resembles
Eq.~(\ref{eq:fitnessbalanceeq}), but with the  effective  {\gain} and {\price} vectors
$\bvtot^{\rm eff} = \bvtot + \Amat_{\rm v}\trans \betav$,
$\hc^{\rm eff} = \hc - \Amat_{\rm c}\trans \betav$, and
$\hu^{\rm eff} = \hu - \Amat_{\rm u}\trans \betav$. These effective
vectors contain  the actual {\gain}s and
{\price}s, as well as  shadow {\myvalue}s and {\price}s due to 
constraints. If many variables hit their constraints, the effective
{\gain} and {\price} vectors will be less sparse than the original
ones. In practice, if the constraints are upper and lower bounds on
the single variables, a flux that hits a lower (or upper) bound will
have an extra positive (or negative) {\gain}. Likewise, each
metabolite or enzyme level that hits a lower (or upper) bound will
have an extra negative (or positive) {\price}.

\subsection{Constraints on enzyme profiles due to kinetics and steady-state condition}
\label{sec:importancereversible} 

So far, in our optimality problems we assumed that cells can freely
vary their enzyme levels and that any enzyme profile leads to a
feasible steady state. This is not always the case: for certain (not
very realistic) rate laws, there exist enzyme profiles that do not
lead to a steady state. This restricts the region of possible enzyme
profiles from which we can choose during optimisation. Figure
\ref{fig:unidirectional} (a) shows an example: in a metabolic pathway
model with irreversible rate laws, the maximal velocities
$k^{\rm cat}_l\,u_l$ must not decrease along the pathway because
otherwise intermediates might accumulate, thus preventing a steady
state. In this case, enzyme profiles will be restricted to some
feasible region in enzyme space. If the optimal enzyme profile is
located on the boundary of this feasible region,
we need to consider Lagrange multipliers  (shadow
{{\enzymeprice}}s) for the boundary constraints, which then appear as terms
in the economic balance
equations.  If one ignores this fact, paradoxical results may arise.
In the model in Figure \ref{fig:unidirectional}, for example, there
can  be enzymes that catalyse a reaction, but have no control over the reaction flux.
\coout{A reversible mass-action kinetics
  $v=u\,\cdot (k_{+} a- k_{-} b)$, for instance, would be allowed, but
  not the irreversible rate law $v = u\, k_{+}\, a$.}  Consider, for
example, a linear pathway with a flux objective (Figure
\ref{fig:unidirectional} (b) and (c)).  If the first reaction has an  
irreversible rate law (and no allosteric regulation), the downstream
enzymes have no flux control, and accordingly, vanishing  {{\enzymebenefit}}s.
Likewise, if one applies a virtual supply flux, this  would lead to an accumulation of
pathway intermediates, but due to irreversibility this would not
slow down the first reaction and so the supply fluxes would directly
add to the pathway flux; this means that all intermediates have the
same economic potential as the end product, which again amounts to vanishing
{\enzymebenefit}s.  This directly leads to a paradox: since
{{\enzymebenefit}}s and costs must be balanced, all enzyme levels
except for the first must vanish, so there cannot even be any flux. So
where is the mistake?

\co{we did not consider constraints on feasible states!} \co{the logic
  here is not so clear .. rewrite, keeping the necessary shadow values
  in mind! maybe this can be very short! jsut say that there is a
  fallacy, and how it can be fixed // and for the graphics, note that
  the constraints are actually EQUALITY, not inequality constraints!}
When numerically optimising an enzyme profile, we may encounter
candidate profiles that would lead to accumulation or depletion of
intermediates. To allow for a steady state, we need to exclude these
regions from enzyme space by applying constraints
(e.g.~$k^{\rm cat}_{i+1}\, u_{i+i} \ge k^{\rm cat}_{i}\,u_i$). The
resulting optimum may be located on the boundary of the allowed
region, as shown in Figure \ref{fig:unidirectional} (a), and the
constraints on this boundary will be associated with Lagrange
multipliers (``negative shadow {\price}s''), which need to be included
in the reaction balance. There are two important cases in which steady
fluxes require fine-tuned enzyme levels (thus constituting a
``kinetic'' enzyme constraint): (i) if an enzyme is fully
substrate-saturated (and so the flux is independent of the substrate
concentration); (ii) if a reaction is fully irreversible (and so the
flux is independent of the product concentration). These constraints
will affect the economic potentials. In case (i), all economic
potentials upstream of the reaction will vanish. In case (ii), all
economic potentials downstream of the reaction will be identical, so
the potential differences vanish. In both cases, a steady state
requires fine-tuned enzyme levels.  Since models with irreversible
rate laws typically show this problem, and since irreversible rate
laws are not physically justified anyway, they should be avoided in
metabolic value theory. In models with only reversible rate laws, these
problems do not arise: each enzyme will have some positive flux
control, and virtual supply fluxes of downstream metabolites
contribute more strongly to the production objective, so the economic
potentials increase along the pathway.

\begin{figure*}[t!]
 \begin{center}
  \includegraphics[width=15cm]{\psfileskinetic/unidirectional_reaction_in_pathway.eps}
 \end{center}
 \caption{\co{state clearly, here and in
     text, the paradox stems from the non-consideration of lagrange
     multipliers! THIS is the problem with irreversible reactions!}
   The usage of irreversible rate laws in models can lead to
   paradoxical results.  (a) Unbranched pathway with identical
   irreversible rate laws in all reactions. In the model, all enzyme
   levels must be fine-tuned to exactly the same level to enable a
   steady state. Any decrease of enzyme levels would lead to an
   infinite accumulation of the enzymes' substrates. Therefore, for a
   steady state to exist, enzyme profiles with decreasing enzyme
   levels along the pathway must be excluded: the remaining feasible
   enzyme profiles forms a polyhedron in enzyme space. \co{eigentlich
     INCREASE ist genauso schlimm. durchdenken!}  The optimal enzyme
   profile is a boundary optimum (red point) within the feasible
   subset, characterised by negative shadow {{\enzymeprice}}s. If one
   ignores this constraint, one may get to paradoxical results like
   the following.  (b) Simple pathway with a flux objective. If the
   first rate law is irreversible, the downstream enzymes have no flux
   control and cannot provide any benefit. In enzyme-optimal states,
   their levels means that there is no flux.  (c) At the same time,
   due to the irreversible reaction, supply fluxes would directly add
   to the pathway flux (instead of slowing down the upstream
   reactions, as usually).  All intermediates have the same economic
   potential as the end product, which again agrees with the vanishing
   enzyme {\myvalue}s between them.}  \coout{Some of these paradoxical
   effects can be prevented by banning irreversible rate laws.}
  \label{fig:unidirectional}
\end{figure*}

\subsection{Leaky expression and soft bounds on enzyme levels.}
\label{sec:boundaryoptimaavoidedleaky}

\co{is mentioned in appendix; also mention this in CBA optimility, bei
  constraints vs costs} In our optimal states, an inactive reaction is
a reaction with a vanishing flux $v_{l}=0$ and an enzyme level
$u_{l}=0$, hitting its lower bound (positivity constraint).  However,
inactive reactions can also be modelled differently. We assume that
enzyme levels cannot be shut down completely, but that, instead, leaky
enzyme expression leads to a small, positive enzyme level
$\varepsilon$, whose complete suppression would be costly.  In a
model, this is expressed by an extra cost term $h^{\rm leak}(\esymbolv)$,
which rises as the enzyme level becomes very small. For instance, we
may set $h^{\rm leak}(\esymbolv)=\sum_{l} \varepsilon^{2}/u_{l}$ yielding
the gradient $h^{\rm leak}_{u_{l}}=-(\varepsilon/u_{l})^{2}$. The new
fitness function, including this cost term, diverges at
$u_{l} \rightarrow 0$. Instead of a boundary optimum at $u_{l} = 0$,
it has an interior optimum with positive (possibly very small) enzyme
levels. This is an example of objective terms and constraints that
have similar effects and that can replace each other in models. Let us
see the resulting balance equation. From the optimality condition
$\mbox{max} \stackrel{!}{=} \gplus(\esymbolv)-\hminus(\esymbolv)-h^{\rm
  leak}(\esymbolv)$, we obtain the cost-benefit balance
\begin{eqnarray}
 \gplus_{u_{l}}-\hul = h^{\rm leak}_{u_{l}} = - (\varepsilon/u_{l})^{2}.
\end{eqnarray}
The cost on the right approaches zero if $u_{l} \gg \varepsilon$ and is
negative otherwise. The resulting flux benefit balance
\begin{eqnarray}
 [\Deltar \wtotl + \bvdirl]\, v_{l} = \hul\,u_{l} - \varepsilon^{2}/u_{l}
\end{eqnarray}
contains a new cost term, which replaces the Lagrange multiplier that would come
with the hard constraint $u_{l}>0$. For the active enzymes, the
cost term $\hul$ dominates, but for inactive enzymes the stress term
becomes important and prevents smaller enzyme levels.

\subsection{Non-optimal states and economic imbalance}
\label{sec:violationsnonenzymatic}

\co{call the imbalance ``opportunity cost''? (THANKS TO RON!) nur hier
  fuer die erklaerung, nicht allgemein!}  The flux benefit balance
equation (\ref{eq:reactionbalanceeq}) states that cost and benefit of
an active enzyme, in optimal states, must be balanced.  Can we use
similar balance equations to also model non-optimal states?  More
commonly, enzymes will show non-optimal levels directly after a
perturbation, when there has not been enough time for adaptation 8or
also after an enzyme knockdown.  To describe non-optimal states, we
assume that the enzymes satisfy an imbalance
\begin{eqnarray}
 \label{eq:knockdown1}
 [\Deltar \wtotl + \bvdirl]\, v_{l} =  \hudotl^{\rm opt} \neq  \hudotl^{\rm real},
\end{eqnarray}
where $\hudotl^{\rm opt}$ is the optimal {\costshade} that would be in
balance with the economic potentials, and $\hudotl^{\rm real}$ is the
actual point cost of the enzyme.  The mismatch -- the difference
$\hudotl^{\rm opt} - \hudotl^{\rm real}$ between optimal and actual
{\enzymecost} is called \emph{economic stress} \co{wort? uea}
$\fudotl$. It is given by
$\fudotl = \partial \ffit/\partial u_{l} = [\Deltar \wtotl +
\bvdirl]\,v_{l} - \hul\,u_{l}$.  Formally, we can replace the
inequality (\ref{eq:knockdown1}) by a reaction balance
\begin{eqnarray}
 \label{eq:knockdown2}
[\Deltar \wtotl + \bvdirl]\, v_{l} = \hudotl^{\rm real} + \fudotl
\end{eqnarray}
with $\fudotl$ as an extra term (Eq.~(\ref{eq:econForceEquation})
in the article.  The economic stress tells us how strongly the flux
benefit balance is violated.  If the enzyme level is too low, the
economic stress will be positive; if the level is too high, it is
negative.  Thus, the inequality states that a change in enzyme level
-- if it were possible -- would be profitable.  The imbalance equation
can also be used in \enzymevalueform
\begin{eqnarray}
\label{eq:econPressureEquation}
\left[ \Deltar \wtotl + \bvdirl \right] \frac{v_{l}}{u_{l}} &=& \hul + \ful
\end{eqnarray}
with enzyme {\myvalue}, enzyme {\price}), and the enzyme
\stress $\ful = \frac{\partial \ffit}{\partial u_{l}}$, and
in the  \fluxvalueform
\begin{eqnarray}
\label{eq:econPressureEquation2}
 \Deltar \wtotl + \bvdirl &=& \hvl + \fvl
\end{eqnarray}
with {\fluxvalue}, flux {\fluxburden}), and the flux
\stress
$\fvl = \frac{1}{v_{l}}\frac{\partial \ffit}{\partial \ln u_{l}}$.

\subsection{Non-enzymatic reactions}
\label{sec:nonenzymatic}

\myparagraph{\ \\Kinetic models with non-enzymatic reactions and
  dilution} So far, we assumed that all reactions are catalysed by
enzymes and are therefore directly controllable.  In reality, there
are also non-enzymatic reactions, ranging from the fast protonation of
acids to the damage of proteins or DNA by reactive oxygen species.
Even metabolites dilution in growing cells can be described as a
non-enzymatic degradation reaction, with linear kinetics and the cell
growth rate $\lambda$ as the rate constant.  In models with
non-enzymatic reactions, the rules of metabolic value theory seem to be
violated: for example, if a pathway product is diluted, and if this
product acts as a catalyst or contributes directly to cell fitness,
the cells needs to constantly reproduce it. In this case, however, the
economic potential rises along the pathway, but then suddenly drops to
zero. Metabolic value theory would normally exclude such behaviour, and
 to account for non-enzymatic reactions and dilution,
some equations need to
be changed. We
consider the system equations
\begin{eqnarray}
 \label{eq:nonenzymaticequations}
 \md \cintv / \md t = \Nenz\, \vvenz + \Nnon\, \vvnon - \lambda\, \cintv
\end{eqnarray}
with separate terms for enzymatic reactions, non-enzymatic reactions,
and dilution (here dilution fluxes are not included in the flux vector
$\vv$). Accordingly, we obtain the flux vector
$\vv = {\vvenz \choose \vvnon}$, the stoichiometric matrix
$\Nint = (\Nenz | \Nnon)$, and the internal elasticity matrix
$\Eunint = {\Eunint^{\rm enz} \choose \Eunint^{\rm non}}$.  The
Jacobian matrix can be split into
$\Mmat_{\lambda} = \Mmat^{\rm enz} + \Mmat^{\rm non} - \lambda\,
\Imat$, with the terms
$\Mmat^{\rm enz} = {\NR}^{\rm enz}\, \Eunint^{\rm enz}\, \Lmat$ (for
enzymatic reactions), $\Mmat^{\rm non} = \NRnon\, \Eunnon\,\Lmat$ (for
non-enzymatic reactions) and $-\lambda\, \Imat$ (for dilution).
Metabolic control coefficients for such models, as well as their
summation and elasticity theorems, are given in SI
\ref{sec:SIproofMCAwithDilution}.

\myparagraph{{\Summationconnectivitycondition} with dilution} In
models with dilution ($\md \cintv / \md t = \Nint\,\vv + \lambda\,\cintv$),
the {\summationconnectivitycondition} read (proof in section
\ref{sec:demandDilution})
\begin{eqnarray}
 \Kint\trans \,\bvtot 
 &=& \Kint\trans\, \hvv \nonumber \\
 \Lmat\trans\, \hc
 + \lambda\,(\Lmat\, {\Mmat_{\lambda}}\inv)\trans\,\hctot
 &=& (\Eunint\,\Lmat)\trans\, \hvv.
\end{eqnarray}
with the {fluxburden} vector $\hvv = \hu \odots \esymbolv \oslashs \vv$.
The {\summationcondition} remains unchanged. The second equation
contains the extra term
$\lambda\,(\Lmat\,{\Mmat_{\lambda}}\inv)\trans\,\hctot$ with the
proximal concentration {\price}
$\hctot = - {\Eunint}\trans\,\bvtot + \hc$.

\myparagraph{{\Summationconnectivitycondition} with non-enzymatic
  reactions} The \summationconnectivitycondition Eq.~(\ref{eq:fitnessbalance2})
and (\ref{eq:fitnessbalance3}) are only valid if all reactions are
active and enzyme-catalysed.  If reactions are inactive, we can simply
omit them from the model.  Non-enzymatic reactions, in contrast, may
considerably change the shape of enzyme-optimal states. On the one
hand, they may produce valuable compounds ``for free''. On the other
hand, they may degrade valuable metabolites, but cannot be simply
switched off by repressing an enzyme. Instead, the cell can compensate
their effects or may control their fluxes indirectly by changing
enzyme levels -- which may again lead to costs.  Even a single
non-enzymatic reaction can drastically change the enzyme-optimal
states in a model. Our \summationconnectivitycondition should capture this
effect, and we shall now see how these modified conditions look
like. For simplicity, we reorder the reactions (first the enzymatic
reactions, then the non-enzymatic reactions) and write the flux vector
as $\vv = {\vv_{\rm enz} \choose \vv_{\rm non} }$. From the
cost-benefit balance (\ref{eq:fitnessbalanceeq}), we obtain the
following \summationconnectivitycondition for active enzymatic reactions (proof
in section \ref{sec:proofnonenzymatic}):
\begin{eqnarray}
 \label{eq:nonenzymatic2}
 \kv \cdot \bvtot  - \kv_{\rm non} \cdot \gvnon &=& 
 \kv_{\rm enz}\trans (\hudotenz \oslashs  \vv_{\rm enz})\\
 \label{eq:nonenzymatic2conc}
\Lmat\trans\,\hc - (\Eunint\,\Lmat)_{{\rm non}}\trans\, \gvnon &=& 
((\Eunint\,\Lmat)_{{\rm enz}})\trans
 (\hudotenz \oslashs \vv_{\rm enz}).
\end{eqnarray}
In the stationary flux mode $\kv$, the subvector $\kv_{\rm enz}$ is
contains the enzymatic reactions.  The {{\enzymecost}} vector
$\hudotenz = \esymbolv \odots \hu)$ refers to enzymatic reactions, and
$\gvnon = [\Deltar {\wint}^{\rm non} + \bvtotnon]$ refers to
non-enzymatic reactions.  The {\summationcondition}
(\ref{eq:nonenzymatic2}) contains an additional term for active
non-enzymatic reactions.  By splitting
$\kv \cdot \bvtot = \kv_{\rm enz} \cdot \bvtotenz + \kv_{\rm non}
\cdot \bvtotnon$, we can rewrite it as
\begin{eqnarray}
 \label{eq:nonenzymatic2a}
 \kv_{\rm enz}\cdot \bvtotenz 
- \kv_{\rm non}\cdot \Deltar {\wint}^{\rm non} &=& 
 \kv_{\rm enz}\trans (\hudot \oslashs  \vv_{\rm enz}) \nonumber \\
\Rightarrow \kv\cdot {\bvtotenz \choose - \Deltar {\wint}^{\rm non}} &=& 
 \kv_{\rm enz}\trans (\hudot \oslashs  \vv_{\rm enz}). 
\end{eqnarray}
Equations (\ref{eq:nonenzymatic2}) and (\ref{eq:nonenzymatic2a})
differ from the usual {\summationcondition} by an extra term, which
describes the effects of non-enzymatic reactions.  here we consider
two special cases: (i) For any flux variation $\modevector$ consisting
of enzymatic reactions, we obtain the original summation
condition. (ii) If we insert a {\flow} $\vv$ as its own flux variation,
Eq.~(\ref{eq:nonenzymatic2}) yields the balance equation
\begin{eqnarray}
 \label{eq:nonenzymatic2b}
 \sum_{l} \hudotl &=& 
 \vv \cdot \bvtot - \vv_{\rm non}\cdot [\Deltar \wvsymbol_{\rm non} + \bvtotnon]\trans.
\end{eqnarray}
In this equation, the total {{\enzymecost}} is not balanced with the
total flux benefit, but with the {\fluxbenefit} minus the
{\fluxbenefit} caused by non-enzymatic reactions. If this extra
term is positive, it will decrease the {\enzymecost}; if it is
negative, the {\enzymecost} increases.  This formula is also valid for
models of growing cells: the dilution ``reactions'' can be treated as
non-enzymatic reactions and can be included into the vector
$\vv_{\rm non}$.

\coout{ \co{If k is {\futile}: $0= \kv_{\rm enz}\trans (\hudot \oslashs 
  \vv_{\rm enz}) + \kv_{\rm non}\trans
  [\Deltar \wvsymbol_{\rm non} + \bvdir_{\rm non}]$ 
 so $\kv_{\rm enz}\trans (\hudot \oslashs  \vv_{\rm enz}) = - \kv_{\rm
  non}\trans [\Deltar \wvsymbol_{\rm non} + \bvdir_{\rm non}]$}

\co{falls $k_{l}= v_{l}$ for all active reactions in $\kv$ then
$\sum_{l} \hudotl$ all active enz reactions in $\kv$ $=\kv_{\rm
 non}\trans [\Deltar \wvsymbol_{\rm non} + \bvdir_{\rm non}]$}

 \co{ALSO REDO THE FOLLOWING:
   \begin{itemize}[leftmargin=5mm]
\item futile submodes (definition and statements) WIE SONST, ABER TEST ODES NUR AUF ENZYMATISCHEN REAKTIONEN. STATEMENT: ECONOMICAL =>
 NO FUTILE SUBMODES. Umgekehrt unklar
\item Statements about flux cost minimisation
\item {\fluxvalue}s, economic potentials, economic loads
\item \co{STIMMT NICHT UNBEDINGT: FORMELN WO? 
Balance equations: show that flux benefit balance stays
  the same, and that the compound balance changes; explain how
  concentrations and fluxes, loads and potentials become entangled}
 \co{We now consider systems in which only some of the reactions are
  catalysed by enzyme and therefore directly controllable via gene
  expression.} \co{The economic imbalance can also be used in this
  case.} If a reaction shows a metabolic flux in the absence of
 enzyme, its balance reads
\begin{eqnarray}
 \label{eq:nonenzymatic4}
 v_{l} [\Deltar \wtotl + \bvdirl] \neq 0 
\end{eqnarray}
with a ``$>$'' sign for beneficial reactions and a ``$<$'' sign for
futile reactions. In both cases, we can replace the inequality by
\co{rename ``economic imbalance'' in the case of non-enzymatic
  reactions? or explain that it's related to a hypothetical case in
  which the reaction is enzymatic with enzyme level =1.}
\begin{eqnarray}
 \label{eq:nonenzymatic6}
 [\Deltar \wtotl + \bvdirl] \, v_{l}= \fudotl
\end{eqnarray}
with a positive or with a negative economic imbalance. \co{explain both cases verbally}
\item \co{Other stuff (see theorems, appendix, proofs ...)}
\end{itemize}
}
}

\section{Control coefficients for metabolite perturbations}
\label{sec:SIvirtualVariations}

Metabolic control coefficients \cite{Heinrich1996, rede:88} describe how
small, virtual perturbations of a reaction rate will affect the steady state of a metabolic system. Here, instead, I consider
virtual perturbations of metabolite concentrations (namely, their production rates
or their concentrations). I determine  control matrices for such
perturbations, show how they are related to the usual control
matrices, and demonstrate that they can be seen as non-orthogonal
projectors, projecting local, initial perturbations to the resulting
long-term changes in metabolic states.

\myparagraph{Control coefficients for perturbations of virtual supply
  fluxes} We consider a kinetic model with $n_{\rm int}$ internal
metabolites. If there are conserved moieties in the model, we choose a
set of $n_{\rm ind}$ independent metabolites and split the
stoichiometric matrix into $\Nint = \Lmat \, \NR$, with an
$n_{\rm int} \times n_{\rm ind}$ link matrix $\Lmat$ and a reduced
stoichiometric matrix $\NR$, whose and rows correspond to the
independent metabolites. We can write $\NR = \Lmatplus \Nint$, where
the matrix $\Lmatplus$ is obtained from an
$n_{\rm int} \times n_{\rm int}$ identity matrix $\Imat$ by selecting
the rows corresponding to independent metabolites; we note that
$\Lmatplus\,\Lmat = \Imat$. The effects of small, virtual supply
fluxes $\virtphiindm$ (for the independent internal metabolites) on
the steady-state concentrations
$\cint_{i}=\csteady_{i}(\esymbolv,\xv,\virtphiindv)$ and steady-state fluxes
$v_{l}=\vsteady_{l}(\esymbolv,\xv,\virtphiindv)$ are described by the new control
matrices $\Ccmat_{\virtphiindv} = \partial \cintv/\partial \virtphiindv$
and $\Cvmat_{\virtphiindv} =\partial \vv/\partial \virtphiindv$, which
can be computed as follows. In the presence of supply fluxes
$\virtphiindv$, the stationarity condition reads
\begin{eqnarray}
 0 &=& \NR \vv +  \virtphiindv.
\end{eqnarray}
By taking derivative with respect to $\virtphiindv$, we obtain
\begin{eqnarray}
\label{eq:statresp}
 0 &=& \NR \frac{\partial \ratev}{\partial \cintv}\, \frac{\partial \cvsteady}{\partial \virtphiindv} 
+ \Imat = \NR\,\Eunint\,\Lmat\,\Ccind_{\virtphiind} + \Imat,
\end{eqnarray}
where $\ratev(\cintv)$ describes the rate laws,
$\cvsteadyind(\virtphiindv)$ denotes the steady-state concentrations
of independent metabolites, and the control matrix
$\Ccind_{\virtphiind} = \partial \cvsteadyind(\virtphiindv)/ \partial
\virtphiindv$ contains their derivatives. The matrix
$\Mmat = \NR\,\Eunint\,\Lmat$, the Jacobian matrix for the independent
internal metabolites, is usually invertible (except for pathological
cases in which $\Eunint$ is rank-deficient). By solving
Eq.~(\ref{eq:statresp}) for $\Ccind_{\virtphiind}$, we obtain
\begin{eqnarray}
 \Ccind_{\virtphiind} = - \Mmat\inv
\end{eqnarray}
and therefore
\begin{eqnarray}
\label{eq:controlbysupplyproof-1}
 \Ccmat_{\virtphiind} &=& \Lmat\, \Ccind_{\virtphiind} = - \Lmat\,\Mmat\inv  \nonumber \\
 \Cvmat_{\virtphiind} &=& \Eunint\, \Ccmat_{\virtphiind} = - \Eunint\, \Lmat\,\Mmat\inv.
\end{eqnarray}
For convenience, we formally define the control
matrices
\begin{eqnarray}
\label{eq:controlbysupplyproof-3}
 \Ccmat_{\virtphi} &=&  \Ccmat_{\virtphiind}\, \Lmatplus \nonumber \\
 \Cvmat_{\virtphi} &=&  \Cvmat_{\virtphiind}\, \Lmatplus,
\end{eqnarray}
to describe  perturbations of all internal metabolites.
By comparing them  to the usual unscaled metabolic control matrices
\cite{rede:88}
\begin{eqnarray}
 \Ccmat &=& - \Lmat\,\Mmat\inv \NR \nonumber \\
 \Cvmat &=& \Imat - \Eunint\, \Lmat\,\Mmat\inv \NR,
\end{eqnarray}
we obtain  the relationships
\begin{eqnarray}
\label{eq:controlbysupplyproof1}
\Ccmat &=& \Ccmat_{\virtphi}\,\Nint \nonumber \\
\Cvmat &=& \Imat + \Cvmat_{\virtphi}\,\Nint.
\end{eqnarray}
\todo{Furthermore, the new control matrices satisfy the identities
\begin{eqnarray}
\label{eq:controlbysupplyproof-2}
 (-\Nint\,\Eunc)\,\Ccmat_{\virtphiind} &=& \Imat \nonumber \\
 (-\Nint)\,\Cvmat_{\virtphiind} &=& \Imat \nonumber.
\end{eqnarray}}

\myparagraph{Control coefficients for concentration perturbations}
Similarly, we can define control matrices for perturbations of
metabolite concentrations.  We consider a steady state with internal
metabolite concentrations $\cintv^{\rm init}$. After a variation of
the concentrations
$\cintv^{\rm init} \rightarrow \cintv^{\rm init}+\delta \virtgammav$,
the system will arrive at a new steady state with concentrations
$\cintv = \cintv^{\rm init}+\delta \cintv$. In models without moiety
conservation, the perturbation $\delta \virtgammav$ has no long-term
\co{sicher? multi-stability? gilt das auf jeden fall fuer dv
  ungefaehr=0?} effect, so $\delta \cintv=0$. In models with moiety
conservation, the perturbation will lead to a stationary concentration
change $\delta \cintv = \Ccmat_{\virtgamma}\,\delta \virtgammav$.  The
control matrix reads (proof in SI \ref{sec:ProofsimplegammaControl})
\begin{eqnarray}
\label{eq:simplegammaControl}
\Ccmat_{\virtgamma} = \Imat -
\Lmat\,(\NR\,\Eunint\,\Lmat)\inv\,\NR\,\Eunint = \Imat + \Ccmat\,\Eunint.
\end{eqnarray}

For the resulting flux changes, we obtain a similar control matrix
$\Cvmat_{\virtgamma} = \Eunint\,\Ccmat_{\virtgamma}$. From
Eq.~(\ref{eq:simplegammaControl}) and $\Gmat\,\Lmat = 0$, we can see
that $\Ccmat_{\virtgamma} \,\Lmat =0$ and
$\Cvmat_{\virtgamma} \,\Lmat =0$. Therefore, the only way in which
concentration perturbations can affect steady-state concentrations or
fluxes is by changing the conserved moiety concentrations.

\begin{figure*}[t!]
 \begin{center}
  \includegraphics[width=15.5cm]{\psfileskinetic/projectors.eps}
 \end{center}
 \caption{The effect of small perturbations on metabolic states can
   described by linear projections.  Vectors describing the initial
   perturbation in flux or concentration space are projected onto
   ``proper'' (i.e.~constraint-respecting) vectors that describe the
   remaining long-term effects. (a) Flux space. Since the matrix
   $(\Kmat | \Eunint\,\Lmat)$ is invertible, flux space can be split
   into the subspaces Im($\Kmat$) (subspace of stationary flux
   perturbations) and Im($\Eunint\,\Lmat$) (subspace of non-stationary
   flux perturbations, caused by concentration changes of independent
   metabolites). An initial (non-stationary) flux perturbation
   $\delta \vv$ can be projected to these two subspaces by the
   projection matrices $\Cvmat$ and $-\Eunint\,\Ccmat$, 
   yielding the components $\deltapar \vv=\Cvmat\,\delta \vv$ and
   $\deltaimproper \vv=- \Eunint \Ccmat\,\delta \vv$. (b) Similar
   projections exist in concentrations space (for details, see text).}
  \label{fig:projectors}
\end{figure*}

\myparagraph{The control coefficient matrices are projectors in flux
  and concentration space} The responses of metabolic systems to
perturbations can be described geometrically as projections in flux or
concentration space. The initial perturbation vectors are projected to
the resulting steady-state changes, and the projectors are related to
the control matrices (see Figure \ref{fig:projectors}). We assume that
the Jacobian matrix $\Mmat = \NR\,\Eunint\,\Lmat$ is invertible
(i.e.~that the elasticity matrix $\Eunint$ has full row rank). Flux
space can be split into the subspaces
${\mathcal M}_{\rm v\parallel} = \mbox{Span}(\Kint)$ spanned by
stationay flux modes and the linearly independent subspace
${\mathcal M}_{\rm v/} = \mbox{Span}(\Eunint\,\Lmat)$ spanned by
reaction velocity perturbations due to perturbations of independent
metabolites. Using the theorems of metabolic control theory,
\begin{eqnarray}
\label{eq:MCAtheorems}
{ \Cvmat \choose \Ccmat}\,(\Kint, \; \Eunint\, \Lmat ) = 
\left(\begin{array}{cc}
\Kint & 0 \\ 0 &  -\Lmat
\end{array}\right),
\end{eqnarray}
we can easily see that the matrices
$\Projvpar = \Cvmat = \Imat + \Eunint\,\Ccmat$ and
$\Projvimproper = -\Eunint\,\Ccmat$ are (non-orthogonal) projectors onto
these subspaces:
\begin{eqnarray}
\label{eq:projector1}
{ \Projvpar \choose \Projvimproper}\,(\Kint, \; \Eunint\, \Lmat ) = 
\left(\begin{array}{cc}
\Kint & 0 \\ 0 &  \Eunint\, \Lmat
\end{array}\right).
\end{eqnarray}
Since the sum of the two projectors yields an identity matrix $\Imat$,
the two subspaces must span the entire flux space. We can also see this
from the fact that the matrix $(\Kmat,\;\Eunc\,\Lmat)$ is quadratic
and all its columns are linearly independent (unless $\Eunc$ is
rank-deficient). A similar projection exists for concentration space.
\co{nee .. eigentlich will ich im konzentrationsraum einen unterraum SENKRECHT auf G und einen unterraum SENKRECHT auf NR E!} Concentration space can be split into subspaces
${\mathcal M}_{\rm c\parallel} = \mbox{Span}(\Gmat\trans)$, spanned by
the coeffient vectors defining the conserved moiety, and the linearly
independent subspace
${\mathcal M}_{\rm c/} = \mbox{Span}((\NR\,\Eunint)\trans)$.  The
matrices $\Projcpar = {\Ccmat_{\virtgamma}}\trans = [\Imat + \Ccmat\,\Eunint]\trans$ and
$\Projcimproper = -[\Ccmat\,\Eunint]\trans$, are (non-orthogonal)
projectors onto these subspaces: \co{beweis ist ok, einfach
  hinschreiben und ausrechnen.}
\begin{eqnarray}
\label{eq:projector1}
{ \Projcpar \choose \Projcimproper }\,(\Gmat\trans, \; (\NR\,\Eunint)\trans) = 
\left(\begin{array}{cc}
\Gmat\trans & 0 \\ 0 &  (\NR\,\Eunint)\trans
\end{array}\right).
\end{eqnarray}
Again, since the sum of the two projectors yields an identity matrix
$\Imat$, the two subspaces must span the entire flux space, and we can
also see this from the fact that the matrix
$(\Gmat\trans, \; (\NR\,\Eunint)\trans)$ is quadratic and has full
rank (unless $\Eunc$ is rank-deficient).  \co{NOCHMAL UEBERLEGEN! der
  projektor ist nicht die kontrollmatrix, sondern die TRANSPONIERTE
  KONTROLLMATRIX!  Similarly, consider a sudden metabolite change
  $\delta \cintv$.  The permanent concentration change (which accounts
  for the changes of conserved moieties) is given by the projection
  $\deltaimproper \cintv = \Projcimproper\,\delta \cintv$, while the
  projection $\deltapar \cintv = \Projcpar\,\delta \cintv$ describes
  the (moiety-conserving) part of the concentration change that will
  be cancelled.} \co{refer to usage in ME (relationships between
  direct and indirect values); or refer to here from there?}

What can we learn from these projections? First, we can apply
  the projections to (physical) perturbations,  splitting them into proper
  (constraint-preserving) and improper (constraint-violating)
  components. A flux perturbation $\delta \vv$ (e.g.~the immediate
  consequence of an enzyme level change) can be split into
\begin{eqnarray}
  \delta \vv = \underbrace{\Cvmat \,\delta \vv}_{\deltapar \vv}
  + \underbrace{(1-\Cvmat)\,\delta \vv}_{\deltaimproper \vv},
\end{eqnarray}
where $\deltapar \vv$ is stationary, i.e.~$\Nint\,\deltapar \vv=0$.
The projection
$\deltaimproper \vv = \Projvimproper\,\delta \vv$, in contrast,
describes the part of the initial flux change that is cancelled by the
system dynamics. 
Likewise a concentration perturbation $\delta \cv$ can can be split
into
\begin{eqnarray}
  \delta \cv = \underbrace{\Ccmat_{\virtgamma} \,\delta \cv}_{\deltapar \cv}
  + \underbrace{(1-\Ccmat_{\virtgamma})\,\delta \cv}_{\deltaimproper \cv},
\end{eqnarray}
where $\deltapar \cv$ is moiety-preserving,
i.e.~$\Gmat\,\deltapar \cv=0$.  Second, we can apply projections to
direct {\myvalue} vectors. The fitness effect of a (possibly
non-stationary) flux perturbation $\delta \vv$ is given by
$\delta \vv\cdot\gvtot$, where \co{note that wv ist auch av!!}
\begin{eqnarray}
\gvtot\trans &=& {\Ccmat}\trans \,\hc + {\Cvmat}\trans\,\bvtot.
\end{eqnarray}
We can see the two terms as projections of $\bvtot$ and
$\hc$. \co{bessere begruendungen, aus projektoreigenschaften!} Given
that $\Ccmat = -\Lmat(\Nint\,\Eunint\,\Lmat)\inv\,\Nint$, the result
of the first term must be in Im(${\Nint}\trans$), and therefore
orthogonal on all stationary flux vectors. On the contrary, given that
$\Cvmat=\Imat-\Eunint\,\Ccmat$, the second term, must be orthogonal on
Im(${\Nint}\trans$), and therefore in the space of stationary flux
vectors. \co{this can be used to correct wv or av obtained from
  empirical data} If we assume that $\delta \vv$ is a stationary flux
variation, the first term must disappear (no effect of metabolite
costs) and the second term is directly given by
$\delta \vv \cdot \bvtot$, because $\Cvmat$ projects $\delta \vv$ onto
itself. \co{entsprechend fur stoerung $\delta \cv$, mit fitness effect
  $\delta \cv \cdot \wtot$ und
  $\wtot\trans = {\Ccmat}\trans_{\virtgamma} \,\hc +
  {\Cvmat}\trans_{\virtgamma}\,\bvtot.$ und entsprechenden
  projektoreigenschaften!}
