# Supplementary material for: Enzyme economy and metabolic control
Source: arXiv:1404.5252 source file (2022-10-04)
Supplement: Supplementary file 2 [file sec_supplement_cba_kinetic_model_construction.tex]

\section{Computing enzyme-optimal states}

\subsection{Economical fluxes computed from {{\enzymecost}}s}
\label{sec:fluxesfromenzymecosts} 

\coout{What is the meaning of the two equations? (i) Stationarity (ii)
  Scaling of flux costs to match the predefined flux benefit (in
  linear chain: only one scaling factor is needed! It is NOT
  considered here in any way that u increases with v (in fact, given
  the overall benefit, a higher y leads to a LOWER v! (remember that y
  are ALREADY assumed to stem from an optimal state; this is where
  further smartness comes in.) A solution yields v, this yields Delta
  v.  If one does not fully trust the $y$ or the relative scaling of y
  and bz, then one can still use the relationship $v = u * kcat * ..$
  to formulate constraints vl <= u kcat, to be used when computing
  v. (if the relative scaling between y and bv is unknown, one may
  predefine y, relate v to y and bv, and treat bv as a variable to be
  minimised.}

If a pathway is known to be in a stationary, enzyme-beneficial state,
and if the {\enzymecost}s and the flux directions in the pathway are
known, this is sufficient information to compute all reaction
fluxes  (we require that the predefined flux signs must be realisable by a  steady
  state). No further knowledge about metabolite concentrations or
kinetics is needed!  The fluxes can be computed from the
{\summationcondition} and from stationarity (proof in
\ref{sec:UniquenessProof}).  In some cases, these equations can be
solved analytically. In Box 1, this is shown for two examples, an
unbranched pathway and a branch point.

\begin{figure*}[t!]
\mybox{
\textbf{Box 1: Computing the metabolic fluxes from {\enzymecost}s}\\

\textbf{Example 1: Linear chain of reactions}\\

\includegraphics[width=15cm]{\psfileskinetic/unbranchedflux.eps}

{\small
\co{symbol y falsch ?? use blue2 for blue text; formeln in c schoener
  (oder in caption?)}  (a) Simple linear chain (with external
metabolites A and B and internal metabolite X). (b) In steady state,
the reactions must show the same flux, $v_{1}=v_{2}$. (c)
{\summationcondition} $\hudotone/v_{1}+\hudottwo/v_{2} = b$ with
${\Kint}=(1,1)\trans$ (unitless) and $\bvtot=(0,b)\trans$, i.e.~a
demand for the production of X$_{2}$. The solutions $\vv$ form a
hyperbola with the asymptotic fluxes $\vv=(\hudotone/b, \infty)\trans$
and $\vv= (\infty, \hudottwo/b)\trans$.  (d) Together, the two
conditions determine the flux.  Two example cases with different
numerical values for {{\enzymecost}}s $\hudotl$ (dark and light blue)
are shown. The calculation for a longer pathway is similar: the
{\summationcondition} with the {\flow} $\kv=(1,1,...,1)\trans$ leads to
the sum rule $\sum_{l} \hudotl/v_{l}=b$. Since all reaction fluxes
must be equal, we obtain
the {\flow} $\vv=(\sum_{l} \hudotl)/b\,\cdot (1,1,...,1)\trans$.\\
 %\label{fig:unbranchedflux}
}

  \textbf{Example 2: Metabolic branch point}\\

  \includegraphics[width=15cm]{\psfileskinetic/branchflux.eps}

  {\small
  \co{in
    d and e, use different colour for the two constraints; give the
    constraints names (in the drawing b)} (a) Metabolic branch point
  (with external metabolites A, B, C and internal metabolite X). (b)
  The {\summationcondition} Eq.~(\ref{eq:fitnessbalance2}),
  $\kv\trans \diag(\hudot)\,\vv\inv = \kv \cdot \bvtot$ implies a
  linear relationship (with an offset) between the inverse fluxes
  $v_{1}\inv$ and $v_{2}\inv$. (c) This yields a nonlinear
  relationship between the fluxes themselves (hyperbola function). (d)
  In the branch point model, there are two such relationships
  (projections on the $v_{1}/v_{2}$ and $v_{1}/v_{3}$ planes shown in
  blue, resulting constraint curve shown in \todo{purple}). (e) By
  intersecting this curve with the plane of stationary fluxes (red),
  we obtain a unique {\flow} (black dot). In the example, we assume
  external metabolite {\myvalue}s $w_{\rm A}=0$,
  $w_{\rm B}=w_{\rm C}=1$ and {{\enzymecost}}s
  $\hudot=(1,1,1)\trans$. With the flux variations
  $\modevector^{(1)}=(1,1,0)\trans$ and
  $\modevector^{(2)}=(1,0,1)\trans$ the {\summationcondition}s read
  $1/v_{1}+1/v_{2} = 1$ and $1/v_{1}+1/v_{3} = 1$. By combining them
  with the stationarity condition $v_{1}=v_{2}+v_{3}$, we obtain the
  flux vector $\vv=(3,3/2,3/2)\trans$.}
 }
\end{figure*}

\subsection{Computing metabolic fluxes from enzyme {\costshade}s} 

If the {\summationcondition} and {\connectivitycondition} cannot be
solved analytically, the {\flow} $\vv$ can be numerically computed as
follows (again, we require that the predefined flux signs must be
realisable by a steady state). We first remove all inactive reactions
from the model (those with zero values in $\hudot$). Then we consider
the {\summationcondition} Eq.~(\ref{eq:fitnessbalance2}) in the form
\begin{eqnarray}
\label{eq:fromcoststofluxes}
 {\Kint}\trans \bvtot = {\Kint}\trans \diag(\hudot) \vv\inv, 
\end{eqnarray}
where the vector $\vv\inv$ contains the reciprocal elements of $\vv$.
The {\summationcondition} yields $n_{\rm st}$ linearly independent
equations for $\vv\inv$ (where $n_{\rm st}$ is the number of
independent stationary flux profiles).  From the stationarity
condition, we further obtain $n_{\rm ind}$ linearly independent
equations for $\vv$ (where $n_{\rm ind}$ is the number of independent
metabolites). So we obtain $n_{\rm ind}+n_{\rm st}$ equations in
total. Since the number of columns of the stoichiometric matrix is
given by the rank $n_{\rm ind}$ of the matrix plus the dimension
$n_{\rm st}$ of the right null space, this matches exactly the total
number of reactions. As shown in section \ref{sec:UniquenessProof},
these equations determine the flux vector $\vv$ uniquely.  To compute
the fluxes in practice, we can use one the two following
methods. 
\begin{enumerate}[leftmargin=5mm]
\item \textbf{Iterative projection} \co{check implementation} Our aim
  is to find a {\flow} with predefined flux directions that satisfies the
  {\summationcondition} Eq.~(\ref{eq:fromcoststofluxes}) and the
  stationarity condition $\Nmat \,\vv=0$. To find such a {\flow}, we
  guess an initial flux distribution (e.g.~with fluxes proportional
  to the enzyme levels), and project it to the nullspace of $\Nint$ to
  make it stationary, while enforcing the correct flux signs by
  constraints.  This operation is a quadratic minimisation problem
  with linear constraints. \co{details see matlab file} Next, we
  compute the reciprocal vector $1/\vv$ and project it to the solution
  space of the {\summationcondition} Eq.~(\ref{eq:fromcoststofluxes})
  \co{how?} to make it economical and compliant with the predefined
  enzyme costs.  This is again a quadratic minimisation problem with
  constraints. if we take the reciprocal values again, the resulting
  {\flow} will not be stationary anymore.  To find a {\flow} that satisfies
  both conditions, we iterate the entire procedure until
  convergence. \co{klappt das praktisch? will it converge? possible
    tricks?: (1) when it starts to converge, start to expand 1/v
    functions as (1-v) (in both spaces) (2) use relaxation terms}
\item \textbf{Minimising the mismatch} In a second, alternative
  method, we ensure stationarity by representing our {\flow} $\vv$
  directly as $\vv = {\Kint}\, \hat \vv$ with some vector $\hat \vv$
  of independent fluxes. We insert this expression into
  Eq.~(\ref{eq:fromcoststofluxes}) and  optimise $\hat \vv$
  numerically by minimising the mismatch between the two sides,
while imposing sign constraints on $\vv = {\Kint}\, \hat \vv$. We determine 
\begin{eqnarray}
\label{eq:fromcoststofluxes2}
 \hat \vv = \argmin_{\hat \vv'} \sum_{i} \left(a_{i} - \sum_{l} \frac{A_{il}}{\sum_{j} K_{lj}\, \hat v'_{j}} \right)^{2}
\end{eqnarray}
with the abbreviations $\av={\Kint}\trans\, \bvtot$ and
$\Amat=\Kmat\, \hudot$, \co{is this convex or anything? ich denke
  nicht} and from the solution we obtain our {\flow} $\vv$. As we saw
before, if Eq.~(\ref{eq:fromcoststofluxes2}) with predefined flux
directions has a solution $\vv$, this solution will be unique.  If our
predefined {{\enzymecost}}s are infeasible (i.e.~numerical values
that cannot be realised by any economical metabolic {\flow}s because
positive costs are assigned to pathways that cannot contribute to the
metabolic benefit or because predefined sign pattern implies that
futile submodes are used), there will be no exact solution, and a
mismatch on the right of Eq.~(\ref{eq:fromcoststofluxes2}) will
remain.
\end{enumerate}

\begin{figure*}[t!]
\begin{center}
\parbox{7cm}{(a)\\
  \includegraphics[width=7cm]{\psfileskinetic/modelreconstruction.eps}}\hspace{15mm}
\parbox{6cm}{(b)\\
    \includegraphics[width=5.7cm]{\psfileskinetic/ycm_pmf_model_construction_atp_prod_aerob_glucose_uniform_mu.eps}\\[3mm]
    \includegraphics[width=5.7cm]{\psfileskinetic/ycm_pmf_model_construction_atp_prod_aerob_glucose_uniform_w.eps}
}
\end{center}
\caption{\co{bild is schoen - in paper zeigen?} Constructing metabolic
  models in enzyme-balanced states.  (a) Algorithm for model
  construction. (i) Given the metabolic network, an economical,
  energetically feasible {\flow}  (e.g.~by applying flux cost
  minimisation). (ii) Consistent economic potentials and
  {{\enzymecost}}s (satisfying the reaction balance) and (iii)
  reaction elasticities and economic loads (satisfying the compound
  balance) are computed as described in SI
  \ref{sec:reconstructionbalanced} and in \cite{lieb:14b}. (iv) The rate
  constants are computed from the reaction elasticities.  (v) By checking solutions
  for dynamic
  and economic stability (the second-order conditions), enzyme-optimal states
  were obtained.   (b) Reconstructed chemical potentials (top)
  and economic potentials (bottom), in yeast central metabolism under
  aerobic conditions. Other ways to construct models in optimal
  states, are described in \cite{lieb:14b,nfbd:16,wnfb:18}.}
  \label{fig:reconstruction}
\end{figure*}

\subsection{Construction of models in enzyme-optimal states}
\label{sec:reconstruction}
\label{sec:reconstructionbalanced}

\coout{rolle von load in construction? o model construction: muss man
  wirklich loads samplen, oder geht es effektiv nur um constraints
  beim elastizitaetssamplen?  echtes samplen noetig, oder geht auch
  samplen von elastizitaeten, + automatisches berechnen von load aus
  potential? kann man mit anderen formeln beim potentialsuchen zc
  schon irgendwie einbeziehen?}

\myparagraph{\ \\Constructing kinetic models in enzyme-balanced
  states} Computing optimal enzyme levels in kinetic models can be
difficult, \co{generally, multiple local optima.  note that FCM with
  enzymetic cost can do this, but it is difficult itself} and it is
even more difficult to obtain solutions with plausible metabolite
concentrations and fluxes.  To construct an enzyme-optimal model with
predefined fluxes, we need to adapt the model parameters, which
drastically increases the numerical effort.  Here I propose an
alternative method: in a first phase, we determine a consistent set of
state variables ($v_{l}$, $\cint_{i}$, $\mu_{i}$, $\Escvlci$, $\bvtotl$,
$\hci$, and $\winti$) and then construct a kinetic model that realises
the state (see Figure \ref{fig:reconstruction}). In this construction,
the state variables $v_{l}$ and $\cint_{i}$, the economic potentials
$\wtoti$ and loads $\loadi$, and the {\gain} and {\price} vectors
$\bvtot$ and $\hc$ must satisfy various conditions, including the
cost-benefit balance, {\gain} conditions, absence of futile submodes,
and the economic balance equations.  In a second phase, we solve for
the necessary kinetic constants.

An algorithm for model construction, based on this concept, is shown
in Figure \ref{fig:reconstruction}. The matrices $\Kint$ and $\Lmat$
are defined by the network, and the {\gain} and {\price} vectors
$\bvtot$ and $\hc$ are also assumed to be predefined.  In the
algorithm, the state variables (fluxes, concentrations, economic
potentials, {{\enzymecost}}s, economic loads, and reaction
elasticities) are chosen step by step, each of them in agreement with
the previous ones. The following criteria must be satisfied: $\vv$
must be stationary, energetically feasible, and pervasive, the
elasticities $\Eunint$ must be consistent with $\vv$ and with the
chemical potentials \cite{liuk:10}, the {\enzymecost}s $\hudotl$ must
be positive, and all economic balance equations must be satisfied.
The algorithm works as follows (for details, see SI
\ref{sec:realisekineticmodels}):

\begin{enumerate}[leftmargin=5mm]
\item \textbf{Steady-state phase} In the steady-state phase, we
  compute an economical metabolic {\flow} $\vv$ together with metabolite
  levels $\cint_{i}$, and economic potentials $\wtoti$ satisfying the
  energetic constraints and the flux benefit balance
  $[\Deltar \wtotl + \bvdirl] \,v_l = \hudotl$. In models with a
  production objective (defined by a vector $\wext$), the {\flow} must be
  free of cyclic submodes; such {\flow}s can be found by
  flux cost minimisation.  Once a {\flow} has been found, the flux
  distribution defines linear constraints for feasible logarithmic
  concentrations and economic potentials. Using these constraints, we
  can use sampling or optimisation with heuristical criteria to determine
  a specific solution $\cintv$, i.e.~concentrations
  $\cint_{i}$, standard chemical potentials $\mu^\circ_{i}$, economic
  potentials $\wint$, and {{\enzymecost}}s $\hudot$ that comply with
  the {\flow}, satisfying the thermodynamic constraints and the economic
  reaction balance.
\item \textbf{Kinetic phase} In the kinetic phase, we choose  the
  economic loads and  kinetic constants in our model. Given  the
  previously determined metabolic state, we search for  reaction
  elasticities $\Escint$ and economic loads that satisfy a compound
  balance Eq.~(\ref{eq:metabolitebalanceequation}) of the form
  $0 = {\Escint}~\trans\, \hudot - \loadint$.  To ensure that our
  reaction elasticities are energetically feasible, we parametrise
  them by saturation values $\beta$ as described in \cite{liuk:10}, and  to
  avoid that  enzymes are fully saturated, we limit the saturation values to a
  certain range, e.g. $0\le \beta_{li}<0.9$.  Moreover, to ensure the
   condition $\Lmat\trans \,\hc = \Lmat\trans \,\loadint$, \co{symbol $\loadint$ gut?} we
  choose internal load vectors of the form
  $\loadint = -\hc + \Gmat\trans \pv^{\rm cm}$.  At first, we  try to
  satisfy these equations for the given vector $\hc$.  Due to our
  previous, arbitrary choice of economic potentials, this may not be
 possible, and if this is the case, we replace $\hc$ by a
  deviation vector $\hc+\hc^{\rm mis}$ and minimise the mismatch
  $\hc^{\rm mis}$ by quadratic programming.  From the resulting saturation
  values, we compute  the elasticities and, finally, all kinetic constants
  for a consistent model.
\end{enumerate}

 Any metabolic state with feasible economic potentials
(determined in the steady-state phase) can be reached by an
enzyme-balanced kinetic model (determined in the kinetic phase). This fact 
is an important theoretical insight. We know that kinetic models
with optimised enzyme levels will satisfy all optimality criteria
listed above. However, does the opposite hold as well?  Can any set of state
variables that satisfy these criteria be  realised by
enzyme-optimal metabolic models?  If this is true, we may choose
steady-state variables -- metabolic fluxes, economic potentials, and
so on -- and construct models that realise these variables.  The
construction algorithm for enzyme-balanced models shows that and how
economical flux distributions can be kinetically realised, and how
this is done in practice.

\myparagraph{Constructing enzyme-optimal models} Toprove that a
metabolic {\flow} is enzyme-optimal (and not only enzyme-balanced), we
need to realise it by a kinetic model in an enzyme-optimal state.  The
state of this model must be both dynamically stable (i.e.~the Jacobian
matrix for independent metabolites must be negative definite) and
economically stable (the fitness curvature matrix must be negative
definite). By sampling the elasticities in the kinetic phase, we
obtain an ensemble of enzyme-balanced models realising the same
metabolic state (see \cite{liuk:10}). If one of them satisfies the
second-order conditions, this proves that the {\flow} is enzyme-optimal,
otherwise the question remains open. The first criterion, dynamical
stability, is not guaranteed by our previous construction, we may
require it as an extra criterion when choosing the reaction
elasticities.  The second criterion, negative fitness curvatures, can
be satisfied by choosing a strongly curved {{\investment}} function
$\hminus(\uv)$, giving rise to a strongly negative curvature matrix
${\bf H}_{\rm uu}$; however, assuming large cost curvatures may be
biologically implausible.

\coout{\subsection{Model of yeast central metabolism}
\label{sec:SIyeast}
The network contains 57 reactions and 68 metabolites, 47 of which are
internal. SI???}
